# Supplementary material for: BF-STVSR: B-Splines and Fourier-Best Friends for High Fidelity Spatial-Temporal Video Super-Resolution
Source: arXiv:2501.11043 source file (2025-03-25)
Supplement: Supplementary file 1 [file X_suppl.tex]

\clearpage
\setcounter{page}{1}
\maketitlesupplementary

%-------------------------------------------------------------------------

\begin{figure*}[!h]
    \centerline{\includegraphics[width=\linewidth]{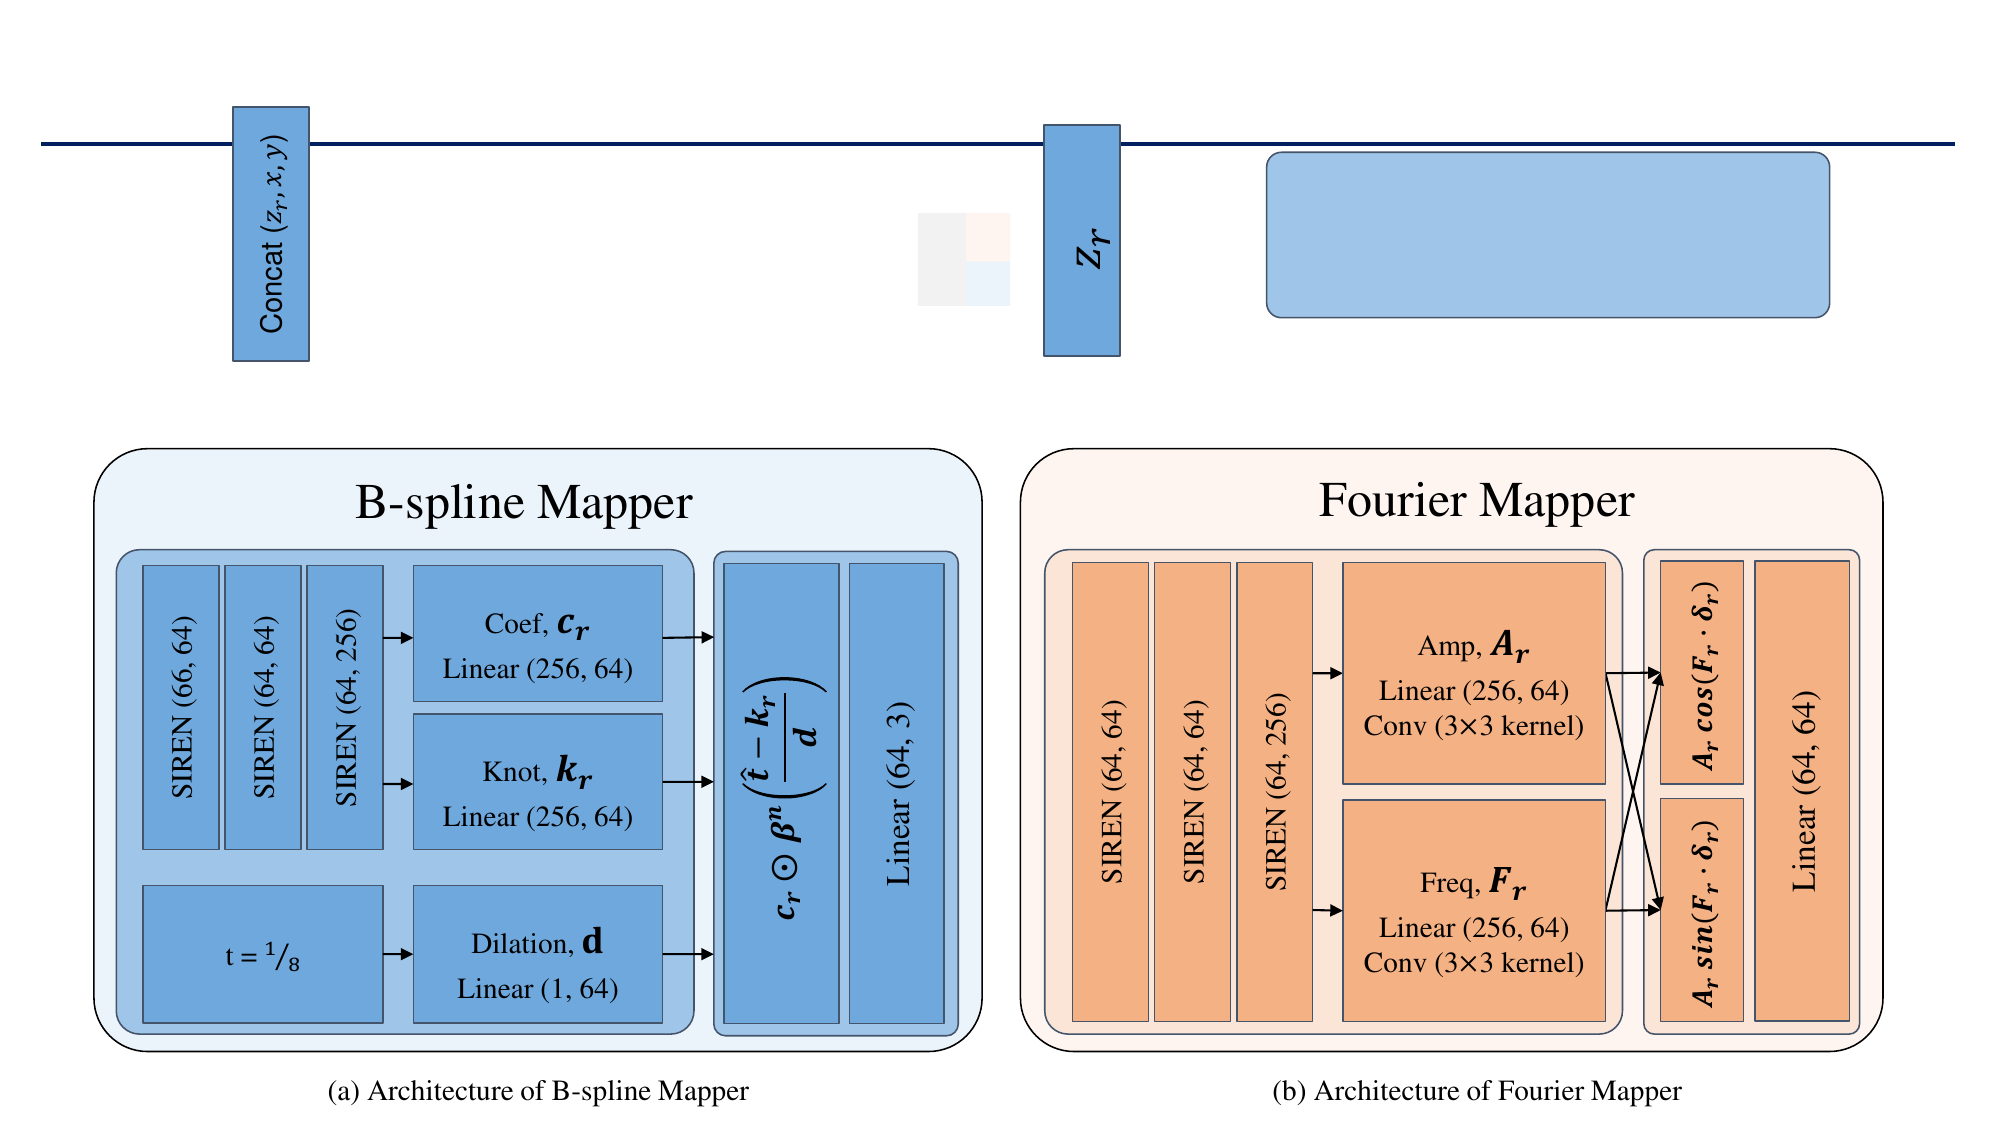}}
    \caption{Detailed Architectures of of {\bspline} and {\fourier}. }
    
    \label{fig_mappers} 
\end{figure*}

%-------------------------------------------------------------------------

\section{Definition of B-spline function}

The B-spline basis function $\beta^n(x)$ is defined as the $n$-fold convolution of $\beta^0(x)$ with itself, where $n$ represents the polynomial degree. The function $\beta^0(x)$ equals 1 when $\vert x\vert < 0.5$ and 0 otherwise. As $n$ increases, the support expands: $\beta^1(x)$ spans $[-1, 1]$, $\beta^2(x)$ spans $[-1.5, 1.5]$, and $\beta^3(x)$ spans $[-2, 2]$. In this study, we adopt the third-order B-spline ($n = 3$) for {\bspline}. The definitions of $\beta^3(x)$ and its derivative $\frac{\partial}{\partial x} \beta^3(x)$ are provided in \Eref{eq:b-spline} and \Eref{eq:b-spline-back}, respectively.

%-------------------------------------------------------------------------
\begin{equation} \label{eq:b-spline}
\beta^3(x) =
\begin{cases} 
\frac{1}{6}(2 + x)^3 & \text{if } -2 < x \leq -1; \\
\frac{1}{6}(4 - 6x^2 - 3x^3) & \text{if } -1 < x \leq 0; \\
\frac{1}{6}(4 - 6x^2 + 3x^3) & \text{if } 0 < x \leq 1; \\
\frac{1}{6}(2 - x)^3 & \text{if } 1 < x \leq 2; \\
0 & \text{otherwise}.
\end{cases}
\end{equation}
\begin{equation} \label{eq:b-spline-back}
\frac{\partial}{\partial x} \beta^3(x) =
\begin{cases} 
\frac{1}{2}(2 + x)^2 & \text{if } -2 < x \leq -1; \\
-2x - 1.5x^2 & \text{if } -1 < x \leq 0; \\
-2x + 1.5x^2 & \text{if } 0 < x \leq 1; \\
-\frac{1}{2}(2 - x)^2 & \text{if } 1 < x \leq 2; \\
0 & \text{otherwise}.
\end{cases}
\end{equation}

%-------------------------------------------------------------------------

\section{Detailed Architectures of Mappers}
We present the detailed network architecture of {\bspline} and {\fourier} in \Fref{fig_mappers}. Both mappers take encoder features as input and capture temporal/spatial information using three-layer SIRENs \cite{siren}. In {\bspline}, a linear layer is used for each coefficient estimator, predicting the coefficients, knots, and dilations for B-spline representations. In {\fourier}, linear and convolutional layers follow the SIREN layers to estimate the amplitudes and frequencies of the Fourier coefficients. Finally, the B-spline or Fourier representations are passed through a linear layer to produce motion vectors or spatial features.

% \section{Additional Results with other basis function.}
\section{Different Position Encodings}

We further compare our model with other position encoding techniques in \Tref{tab:basisfunc}. Specifically, we compare our model with Fourier Encoding (FE) \cite{mildenhall2020nerf}, Thin-Plate Spline (TPS) \cite{zhao2022thin}, which is proved effective in image animation, and Gaussian function ($\simeq\infty$-order B-spline). For FE, we concatenate encoded coordinates with INR input features. For fair comparison, we follow the training scheme of MoTIF \cite{chen2023motif}, which includes the optical flow supervision from the RAFT \cite{teed2020raft}. For Gaussian, similar to ours, we learn scaling, mean, and variance factor. Ours model achieves the best performance, with other basis functions outperformed FE that solely relies on coordinates rather than leveraging priors of basis functions to focus on informative video details.

\begin{table}[h]
\centering
\caption{Performance comparison of different position encodings on GoPro and Adobe240 datasets. Results are evaluated using PSNR (dB) and SSIM metrics. All frames are interpolated by a factor of $\times 4$ in the spatial axis and $\times 8$ in the temporal axis. FE denotes Fourier Encoding and TPS denotes Thin-Plate Spline. \textcolor{red}{Red} indicates the best performance.} 
\label{tab:table2}
% \resizebox{0.8\textwidth}{!}{%
\resizebox{\columnwidth}{!}{
\begin{tabular}{c|cccc}
\hline
\multirow{2}{*}{Method}  & \multicolumn{4}{c}{Test Dataset} \\ 
% \hline
\cline{2-5}
 & Adobe-\textit{Average} & Adobe-\textit{Center}  & GoPro-\textit{Average} & GoPro-\textit{Center} \\ 
\hline
\hline
MoTIF (w FE) & 30.02 / 0.8781 & 30.73 / 0.8855 & 30.08 / 0.8780 & 31.01 / 0.8877 \\

MoTIF (w learnable FE) & 30.05 / 0.8789  & 30.76 / 0.8862 & 30.11 / 0.8786 & 31.06 / 0.8884 \\

MoTIF (w TPS) & 30.02 / 0.8786 & 30.70 / 0.8856 & 30.10 / 0.8783 & 31.03 / 0.8880 \\

BF-STVSR (w gaussian) &  30.06 / 0.8787 & 30.71 / 0.8855  & 30.11 / 0.8777 & 31.01 / 0.8870 \\

% RAFT loss 있는 원래 페이퍼 결과
BF-STVSR + $\mathcal L_{RAFT}$ (Ours) & \textcolor{red}{30.14 / 0.8808} & \textcolor{red}{30.84} / 0.8877 & 30.20 / 0.8799 & 31.14 / 0.8893 \\

% RAFT loss 없는 업데이트 결과
BF-STVSR (Ours) & 30.12 / \textcolor{red}{0.8808} & 30.83 / \textcolor{red}{0.8880} & \textcolor{red}{30.22 / 0.8802} & \textcolor{red}{31.17 / 0.8898} \\

\hline

\end{tabular}%
% }
}
\label{tab:basisfunc}
\end{table}

%%%%%%%%%%%%%%%%%%%%%%%%%%%%%% Version Red %%%%%%%%%%%%%%%%%%%%%%%%%%%%%%
% ------------------------------------------------------

\section{Different Basis Function Configurations}

We conduct additional experiments by varying the basis functions used for both axes in \Tref{tab:ablation2_}. In all configurations, the basis function model the spatial and temporal axes, while other components (\textit{e.g.}, linear projection for intermediate motion vectors and reliability maps) remain the same. Here, we follow the training scheme of MoTIF \cite{chen2023motif}, which incorporating the optical flow supervision in Eq. (5) of the main paper. Although the performance differences among these configurations are minimal, we adopt the configuration using B-spline for temporal representation and Fourier for spatial representation, as it achieves the highest performance. 

% %%%%%%%%%%%%%%%%%%%%%%%%%%%%% Version Bold %%%%%%%%%%%%%%%%%%%%%%%%%%%%%%

% \begin{table}[h]
% \centering
% \caption{Performance comparison on the cross basis function configurations. Results are evaluated using PSNR (dB) and SSIM metrics. ``Ours-cross'' uses {\fourier} as temporal basis function and {\bspline} as spatial basis function. ``Ours-FF'' applies the {\fourier} for both spatial and temporal axes and ``Ours-BB'' employs the {\bspline} for both axes. \textbf{Bold} indicates the best performance.}
% \label{tab:ablation2_}
% \resizebox{\columnwidth}{!}{%
% \begin{tabular}{c|cccc}
% \hline
%  & GoPro-\textit{Center} & GoPro-\textit{Average} & Adobe-\textit{Center} & Adobe-\textit{Average} \\
% \hline
% Ours     & \textbf{31.14} / 0.8893 & \textbf{30.20} / \textbf{0.8799} & \textbf{30.84} / 0.8877 & \textbf{30.14} / 0.8808   \\
% Ours-cross  & 31.10 / 0.8892 & 30.17 / 0.8796 & 30.80 / 0.8876 & 30.10 / 0.8804   \\
% Ours-FF     & 31.12 / \textbf{0.8894} & 30.18 / 0.8798 & \textbf{30.84} / \textbf{0.8879} & 30.13 / \textbf{0.8809}   \\
% Ours-BB     & 31.07 / 0.8885 & 30.16 / 0.8793 & 30.77 / 0.8865 & 30.09 / 0.8797   \\
% \hline
% \end{tabular}%
% }
% \end{table}

% %%%%%%%%%%%%%%%%%%%%%%%%%%%%% Version Bold %%%%%%%%%%%%%%%%%%%%%%%%%%%%%%

%%%%%%%%%%%%%%%%%%%%%%%%%%%%%% Version Red %%%%%%%%%%%%%%%%%%%%%%%%%%%%%%

\begin{table}[h]
\centering
\caption{Performance comparison on the cross basis function configurations. Results are evaluated using PSNR (dB) and SSIM metrics. ``Ours-cross'' uses {\fourier} as temporal basis function and {\bspline} as spatial basis function. ``Ours-FF'' applies the {\fourier} for both spatial and temporal axes and ``Ours-BB'' employs the {\bspline} for both axes. \textcolor{red}{Red} indicates the best performance.}
\label{tab:ablation2_}
\resizebox{\columnwidth}{!}{%
\begin{tabular}{c|cccc}
\hline
 & GoPro-\textit{Center} & GoPro-\textit{Average} & Adobe-\textit{Center} & Adobe-\textit{Average} \\
\hline
Ours     & \textcolor{red}{31.14} / 0.8893 & \textcolor{red}{30.20} / \textcolor{red}{0.8799} & \textcolor{red}{30.84} / 0.8877 & \textcolor{red}{30.14} / 0.8808   \\
Ours-cross  & 31.10 / 0.8892 & 30.17 / 0.8796 & 30.80 / 0.8876 & 30.10 / 0.8804   \\
Ours-FF     & 31.12 / \textcolor{red}{0.8894} & 30.18 / 0.8798 & \textcolor{red}{30.84} / \textcolor{red}{0.8879} & 30.13 / \textcolor{red}{0.8809}   \\
Ours-BB     & 31.07 / 0.8885 & 30.16 / 0.8793 & 30.77 / 0.8865 & 30.09 / 0.8797   \\
\hline
\end{tabular}%
}
\end{table}

%%%%%%%%%%%%%%%%%%%%%%%%%%%%% Version Red %%%%%%%%%%%%%%%%%%%%%%%%%%%%%%

%-------------------------------------------------------------------------

\section{Additional Results on Vimeo90K}

%-------------------------------------------------------------------------

% %%%%%%%%%%%%%%%%%%%%%%%%%%%%%% Version Bold %%%%%%%%%%%%%%%%%%%%%%%%%%%%%%
% \begin{table}[t!]
% \centering
% \caption{Performance comparison on the C-STVSR baselines on Vimeo90K dataset. Results are evaluated using PSNR (dB) and SSIM metrics. All frames are interpolated by a factor of $\times 4$ in the spatial axis and $\times 6$ in the temporal axis. \textbf{Bold} indicates the best performance.}
% \label{tab:table1}
% % \resizebox{0.8\textwidth}{!}{%
% \resizebox{\columnwidth}{!}{
% \begin{tabular}{c|ccc}
% \hline
% \multirow{2}{*}{Method}  & \multicolumn{3}{c}{Test Dataset} \\ 
% % \hline
% \cline{2-4}
%  & Vimeo-\texttt{Fast} & Vimeo-\texttt{Medium} & Vimeo-\texttt{Slow} \\ 
% \hline
% \hline
%  VideoINR \cite{chen2022vinr} & 25.79 / 0.7980 & 28.37 / 0.8553 & 29.25 / 0.8727 \\

%  MoTIF \cite{chen2023motif} & 26.03 / 0.7909 & 28.68 / 0.8574 & 29.47 / 0.8739 \\

%  BF-STVSR + $\mathcal L_{RAFT}$ (Ours) & \textbf{26.53 / 0.8079}  & 28.76 / \textbf{0.8594} & 29.53 / 0.8748 \\

%  BF-STVSR (Ours) & 26.52 / 0.8054  & \textbf{28.77} / 0.8590 & \textbf{29.55 / 0.8750} \\
% \hline

% \end{tabular}%
% % }
% }
% \end{table}

% %%%%%%%%%%%%%%%%%%%%%%%%%%%%%% Version Bold %%%%%%%%%%%%%%%%%%%%%%%%%%%%%%

%%%%%%%%%%%%%%%%%%%%%%%%%%%%%% Version Red %%%%%%%%%%%%%%%%%%%%%%%%%%%%%%
\begin{table}[t!]
\centering
\caption{Performance comparison on the C-STVSR baselines on Vimeo90K dataset. Results are evaluated using PSNR (dB) and SSIM metrics. All frames are interpolated by a factor of $\times 4$ in the spatial axis and $\times 6$ in the temporal axis. \textcolor{red}{Red} indicates the best performance.}
\label{tab:table1}
% \resizebox{0.8\textwidth}{!}{%
\resizebox{\columnwidth}{!}{
\begin{tabular}{c|ccc}
\hline
\multirow{2}{*}{Method}  & \multicolumn{3}{c}{Test Dataset} \\ 
% \hline
\cline{2-4}
 & Vimeo-\texttt{Fast} & Vimeo-\texttt{Medium} & Vimeo-\texttt{Slow} \\ 
\hline
\hline
 VideoINR \cite{chen2022vinr} & 25.79 / 0.7980 & 28.37 / 0.8553 & 29.25 / 0.8727 \\

 MoTIF \cite{chen2023motif} & 26.03 / 0.7909 & 28.68 / 0.8574 & 29.47 / 0.8739 \\

 BF-STVSR + $\mathcal L_{RAFT}$ (Ours) & \textcolor{red}{26.53 / 0.8079}  & 28.76 / \textcolor{red}{0.8594} & 29.53 / 0.8748 \\

 BF-STVSR (Ours) & 26.52 / 0.8054  & \textcolor{red}{28.77} / 0.8590 & \textcolor{red}{29.55 / 0.8750} \\
\hline

\end{tabular}%
% }
}
\end{table}

%%%%%%%%%%%%%%%%%%%%%%%%%%%%%% Version Red %%%%%%%%%%%%%%%%%%%%%%%%%%%%%%

We further evaluate C-STVSR baselines, including VideoINR \cite{chen2022vinr}, MoTIF \cite{chen2023motif}, BF-STVSR + $\mathcal L_{RAFT}$ and BF-STVSR, all trained on Adobe240 dataset, using the Vimeo90K dataset. Vimeo90K, a widely used benchmark for video enhancement, comprises 64,612 clips, each containing seven frames. Following \cite{xiang2020zooming}, we categorize the testset into three motion groups: \texttt{Fast}, \texttt{Medium}, and \texttt{Slow}. The evaluation results, presented in \Tref{tab:table1}, show that our model achieves higher PSNR across all motion categories. Notably, it outperforms VideoINR by approximately 0.7 dB and MoTIF by 0.5 dB on the Vimeo-\texttt{Fast} subset, highlighting its superior ability to effectively handle motion dynamics, even in challenging scenarios.
%-------------------------------------------------------------------------

%%%%%%%%%%%%%%%%%%%%%%%%%%%%%% Version Bold %%%%%%%%%%%%%%%%%%%%%%%%%%%%%%

% \begin{table}[t!]
% \centering
% \caption{Performance comparison on the C-STVSR baselines on GoPro and Adobe240 datasets. Baseline models are trained on Vimeo90K septuplet dataset. Results are evaluated using PSNR (dB) and SSIM metrics. All frames are interpolated by a factor of $\times 4$ in the spatial axis and $\times 8$ in the temporal axis. \textbf{Bold} indicates the best performance.}
% \label{tab:table2}
% % \resizebox{0.8\textwidth}{!}{%
% \resizebox{\columnwidth}{!}{
% \begin{tabular}{c|cccc}
% \hline
% \multirow{2}{*}{Method}  & \multicolumn{4}{c}{Test Dataset} \\ 
% % \hline
% \cline{2-5}
%  & Adobe-\textit{Average} & Adobe-\textit{Center}  & GoPro-\textit{Average} & GoPro-\textit{Center} \\ 
% \hline
% \hline
%  VideoINR \cite{chen2022vinr} & 28.95 / 0.8527 & 29.58 / 0.8603 & 29.43 / 0.8657 & 30.20 /  0.8751 \\

%  MoTIF \cite{chen2023motif} &  28.81 / 0.8495 & 29.47 / 0.8580 & 29.44 / 0.8649 & 30.24 / 0.8742 \\

%  BF-STVSR + $\mathcal L_{RAFT}$ (Ours) & \textbf{29.30 / 0.8611}  & \textbf{29.88 / 0.8677} & \textbf{29.75 / 0.8709} & \textbf{30.53 / 0.8796} \\
% \hline

% \end{tabular}%
% % }
% }
% \end{table}

% %%%%%%%%%%%%%%%%%%%%%%%%%%%%%% Version Bold %%%%%%%%%%%%%%%%%%%%%%%%%%%%%%

%%%%%%%%%%%%%%%%%%%%%%%%%%%%%% Version Red %%%%%%%%%%%%%%%%%%%%%%%%%%%%%%

\begin{table}[t!]
\centering
\caption{Performance comparison on the C-STVSR baselines on GoPro and Adobe240 datasets. Baseline models are trained on Vimeo90K septuplet dataset. Results are evaluated using PSNR (dB) and SSIM metrics. All frames are interpolated by a factor of $\times 4$ in the spatial axis and $\times 8$ in the temporal axis. \textcolor{red}{Red} indicates the best performance.}
\label{tab:table2}
% \resizebox{0.8\textwidth}{!}{%
\resizebox{\columnwidth}{!}{
\begin{tabular}{c|cccc}
\hline
\multirow{2}{*}{Method}  & \multicolumn{4}{c}{Test Dataset} \\ 
% \hline
\cline{2-5}
 & Adobe-\textit{Average} & Adobe-\textit{Center}  & GoPro-\textit{Average} & GoPro-\textit{Center} \\ 
\hline
\hline
 VideoINR \cite{chen2022vinr} & 28.95 / 0.8527 & 29.58 / 0.8603 & 29.43 / 0.8657 & 30.20 /  0.8751 \\

 MoTIF \cite{chen2023motif} &  28.81 / 0.8495 & 29.47 / 0.8580 & 29.44 / 0.8649 & 30.24 / 0.8742 \\

 BF-STVSR + $\mathcal L_{RAFT}$ (Ours) & \textcolor{red}{29.30 / 0.8611}  & \textcolor{red}{29.88 / 0.8677} & \textcolor{red}{29.75 / 0.8709} & \textcolor{red}{30.53 / 0.8796} \\
\hline

\end{tabular}%
% }
}
\end{table}

%%%%%%%%%%%%%%%%%%%%%%%%%%%%%% Version Red %%%%%%%%%%%%%%%%%%%%%%%%%%%%%%

%-------------------------------------------------------------------------
Additionally, we train the C-STVSR models (VideoINR, MoTIF, and BF-STVSR + $\mathcal L_{RAFT}$) using the Vimeo90K trainset until 450K training iterations. Similar to the Adobe240 dataset, we select seven consecutive frames from each video clip, use the $1^{st}$ and $7^{th}$ frames as input reference frames, and randomly sample three intermediate frames as ground-truth. These models are then evaluated on GoPro and Adobe240 datasets, following the \textit{-Center} and \textit{-Average} evaluation protocols detailed in the main paper. The results, presented in \Tref{tab:table2}, demonstrate that our model consistently achieves higher PSNR across all datasets, with improvements of approximately 0.4 dB over VideoINR and 0.3 dB over MoTIF.

These results suggest that our model is both robust and versatile. While trained on specific datasets, it shows promising generalization across diverse datasets, achieving competitive performance in reconstructing high-quality frames. In comparison, previous methods exhibit some challenges in adapting to unseen data, highlighting the potential advantages of our approach.

\section{Additional Qualitative Results}

We provide more qualitative comparison between BF-STVSR and prior methods (VideoINR \cite{chen2022vinr}, MoTIF \cite{chen2023motif}), all trained on Adobe240 dataset. \Fref{figure_x6} and \Fref{figure_x8} present temporal interpolation results (with the spatial scale fixed at 1) on the DAVIS dataset across all temporal coordinates, which were not shown in the main paper, at both the out-of-distribution scale ($\times 6$) and in-distribution scale ($\times 8$), respectively. \Fref{figure_gopro_x4x8} shows the spatial-temporal interpolation results on GoPro dataset at in-distribution temporal scale ($\times 8$) and in-distribution spatial scale ($\times 4$). \Fref{figure_vimeo_medium_x1x6} shows the temporal interpolation results on the Vimeo-\texttt{Medium} testset at the out-of-distribution scale ($\times 6$). \Fref{figure_vimeo_fast_x2x6} and \Fref{figure_vimeo_fast_x4x6} show spatial-temporal interpolation results on the Vimeo-\texttt{Fast} testset at the out-of-distribution temporal scale ($\times 6$) and both out-of-distribution and in-distribution spatial scales ($\times 2$, $\times 4$), respectively.

{
    \small
    \bibliographystyle{ieeenat_fullname}
    \bibliography{suppl}
}

%-------------------------------------------------------------------------

%-------------------------------------------------------------------------

% %-------------------------------------------------------------------------
% \begin{figure}[p]
% \centering
% \includegraphics[width=\textwidth]{your-image-file.png} % Replace with your file name
% \caption{Your caption here.}
% \label{fig:your-label}
% \end{figure}
% \clearpage

\begin{figure*}[!t]
    \centerline{\includegraphics[width=\linewidth]{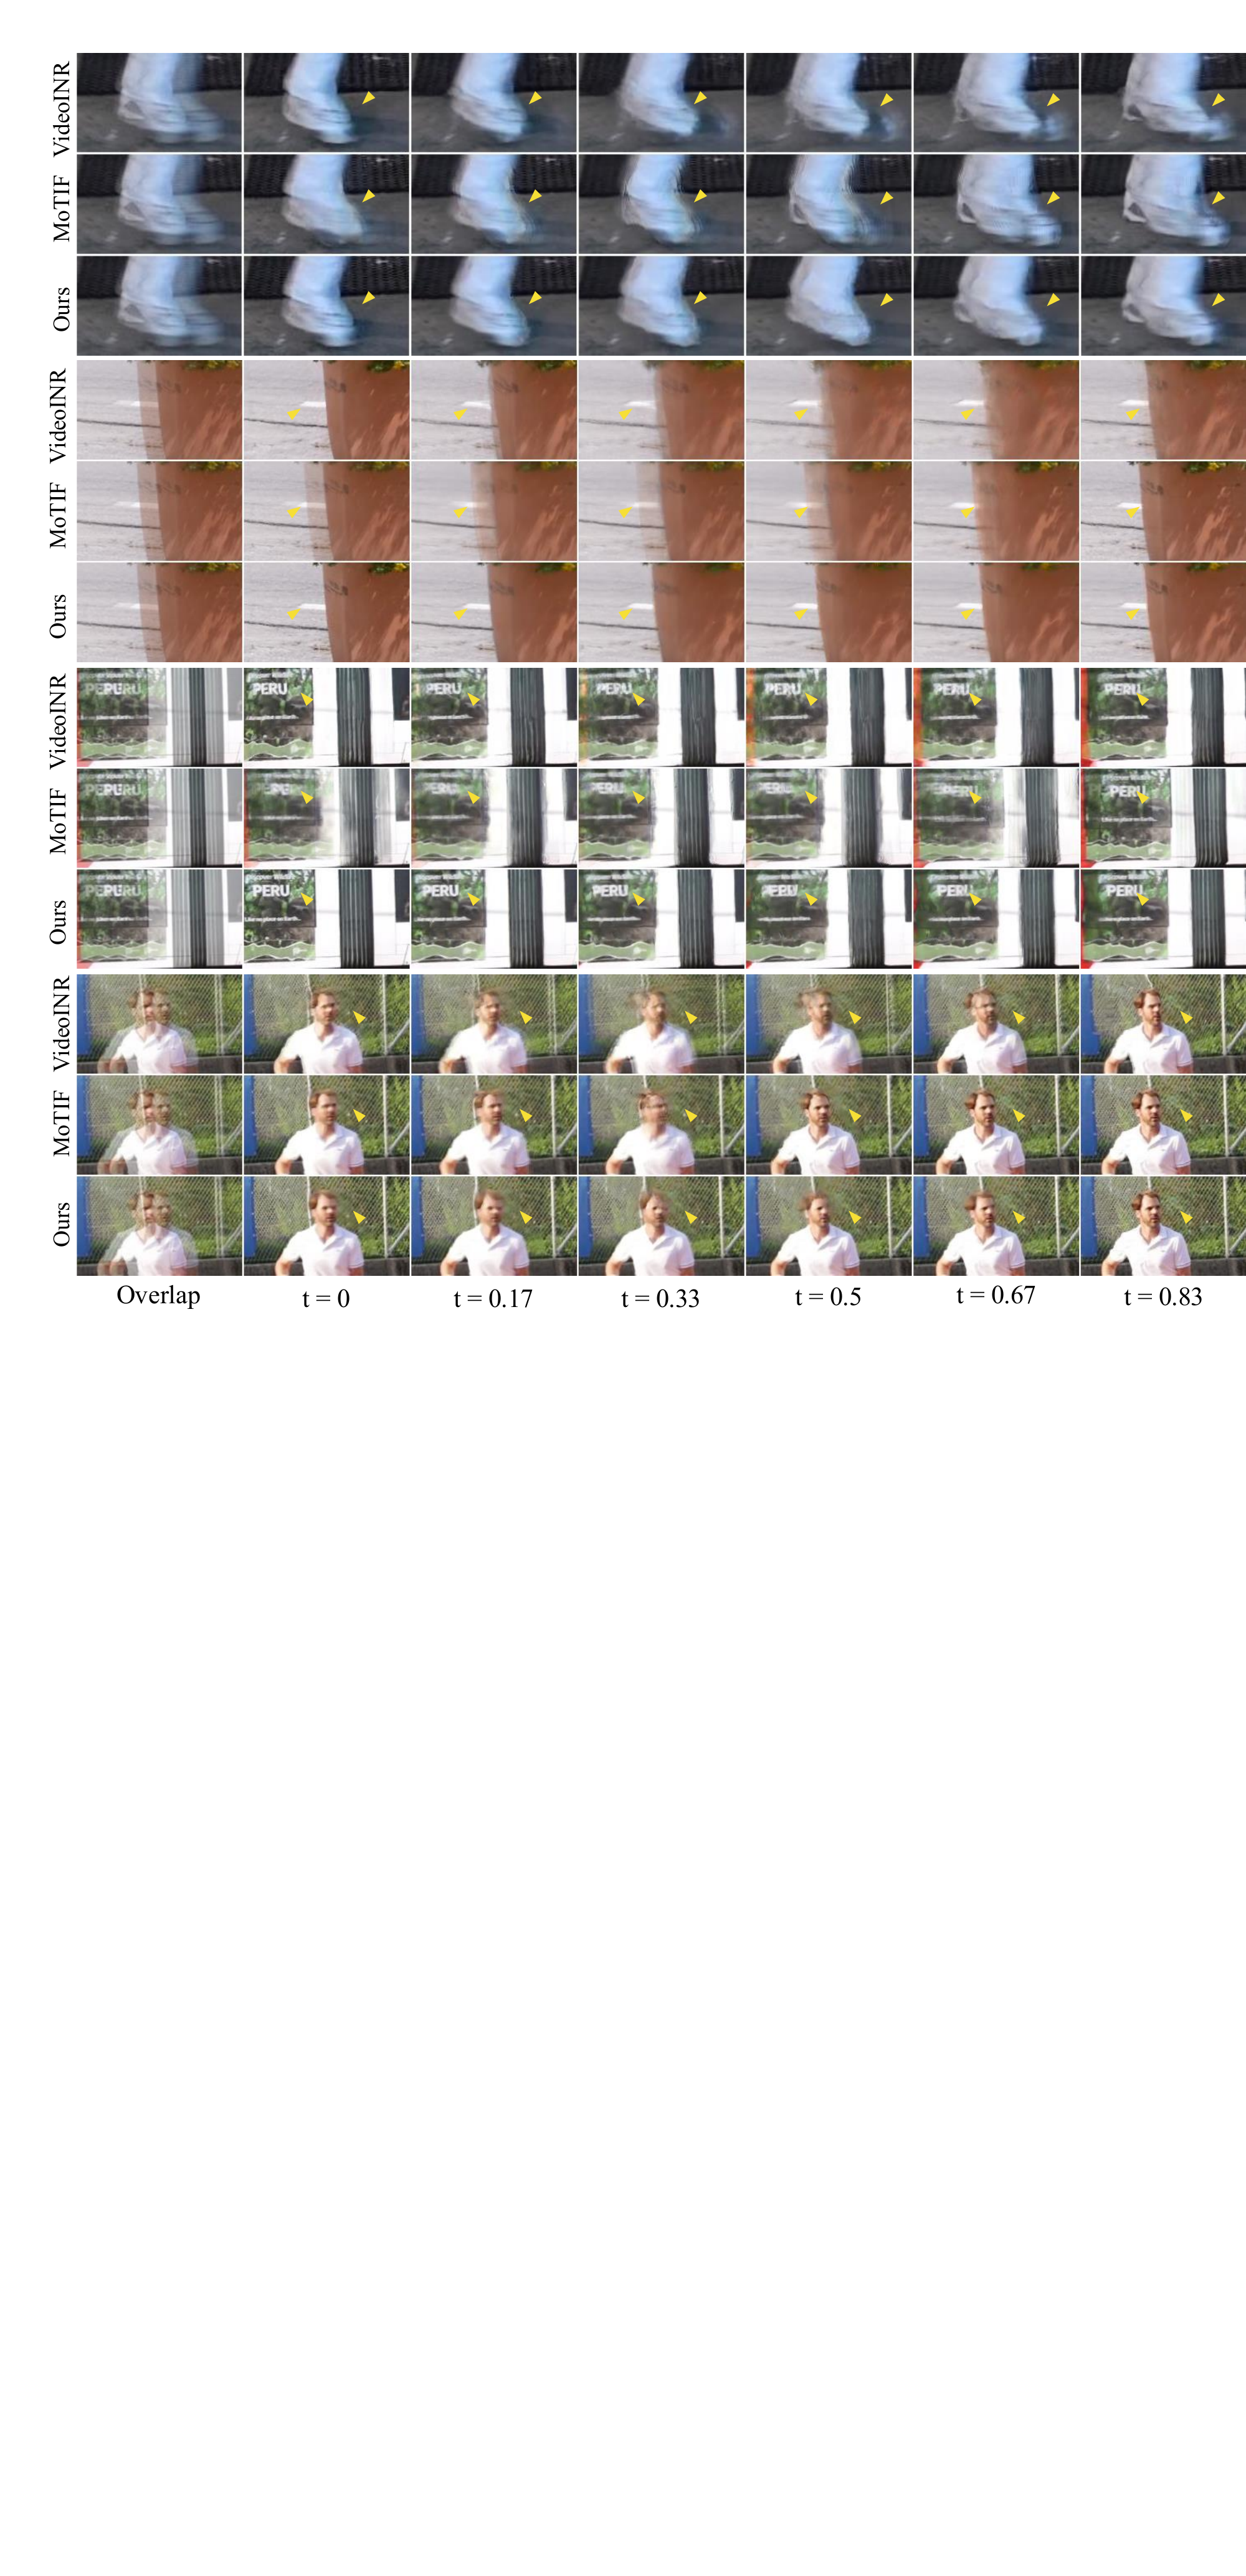}}
    \caption{Qualitative comparison on arbitrary scale temporal interpolation on out-of-distribution ($\times$6) with all time coordinates. We use the DAVIS dataset for evaluation. ``Overlap'' refers to the averaged image of two input frames ($t=0,1$), and the following images are interpolation results at $t=(0,1)$.  }
    
    \label{figure_x6} 
\end{figure*}
\clearpage

%-------------------------------------------------------------------------

\begin{figure*}[!t]
    \centerline{\includegraphics[width=\linewidth]{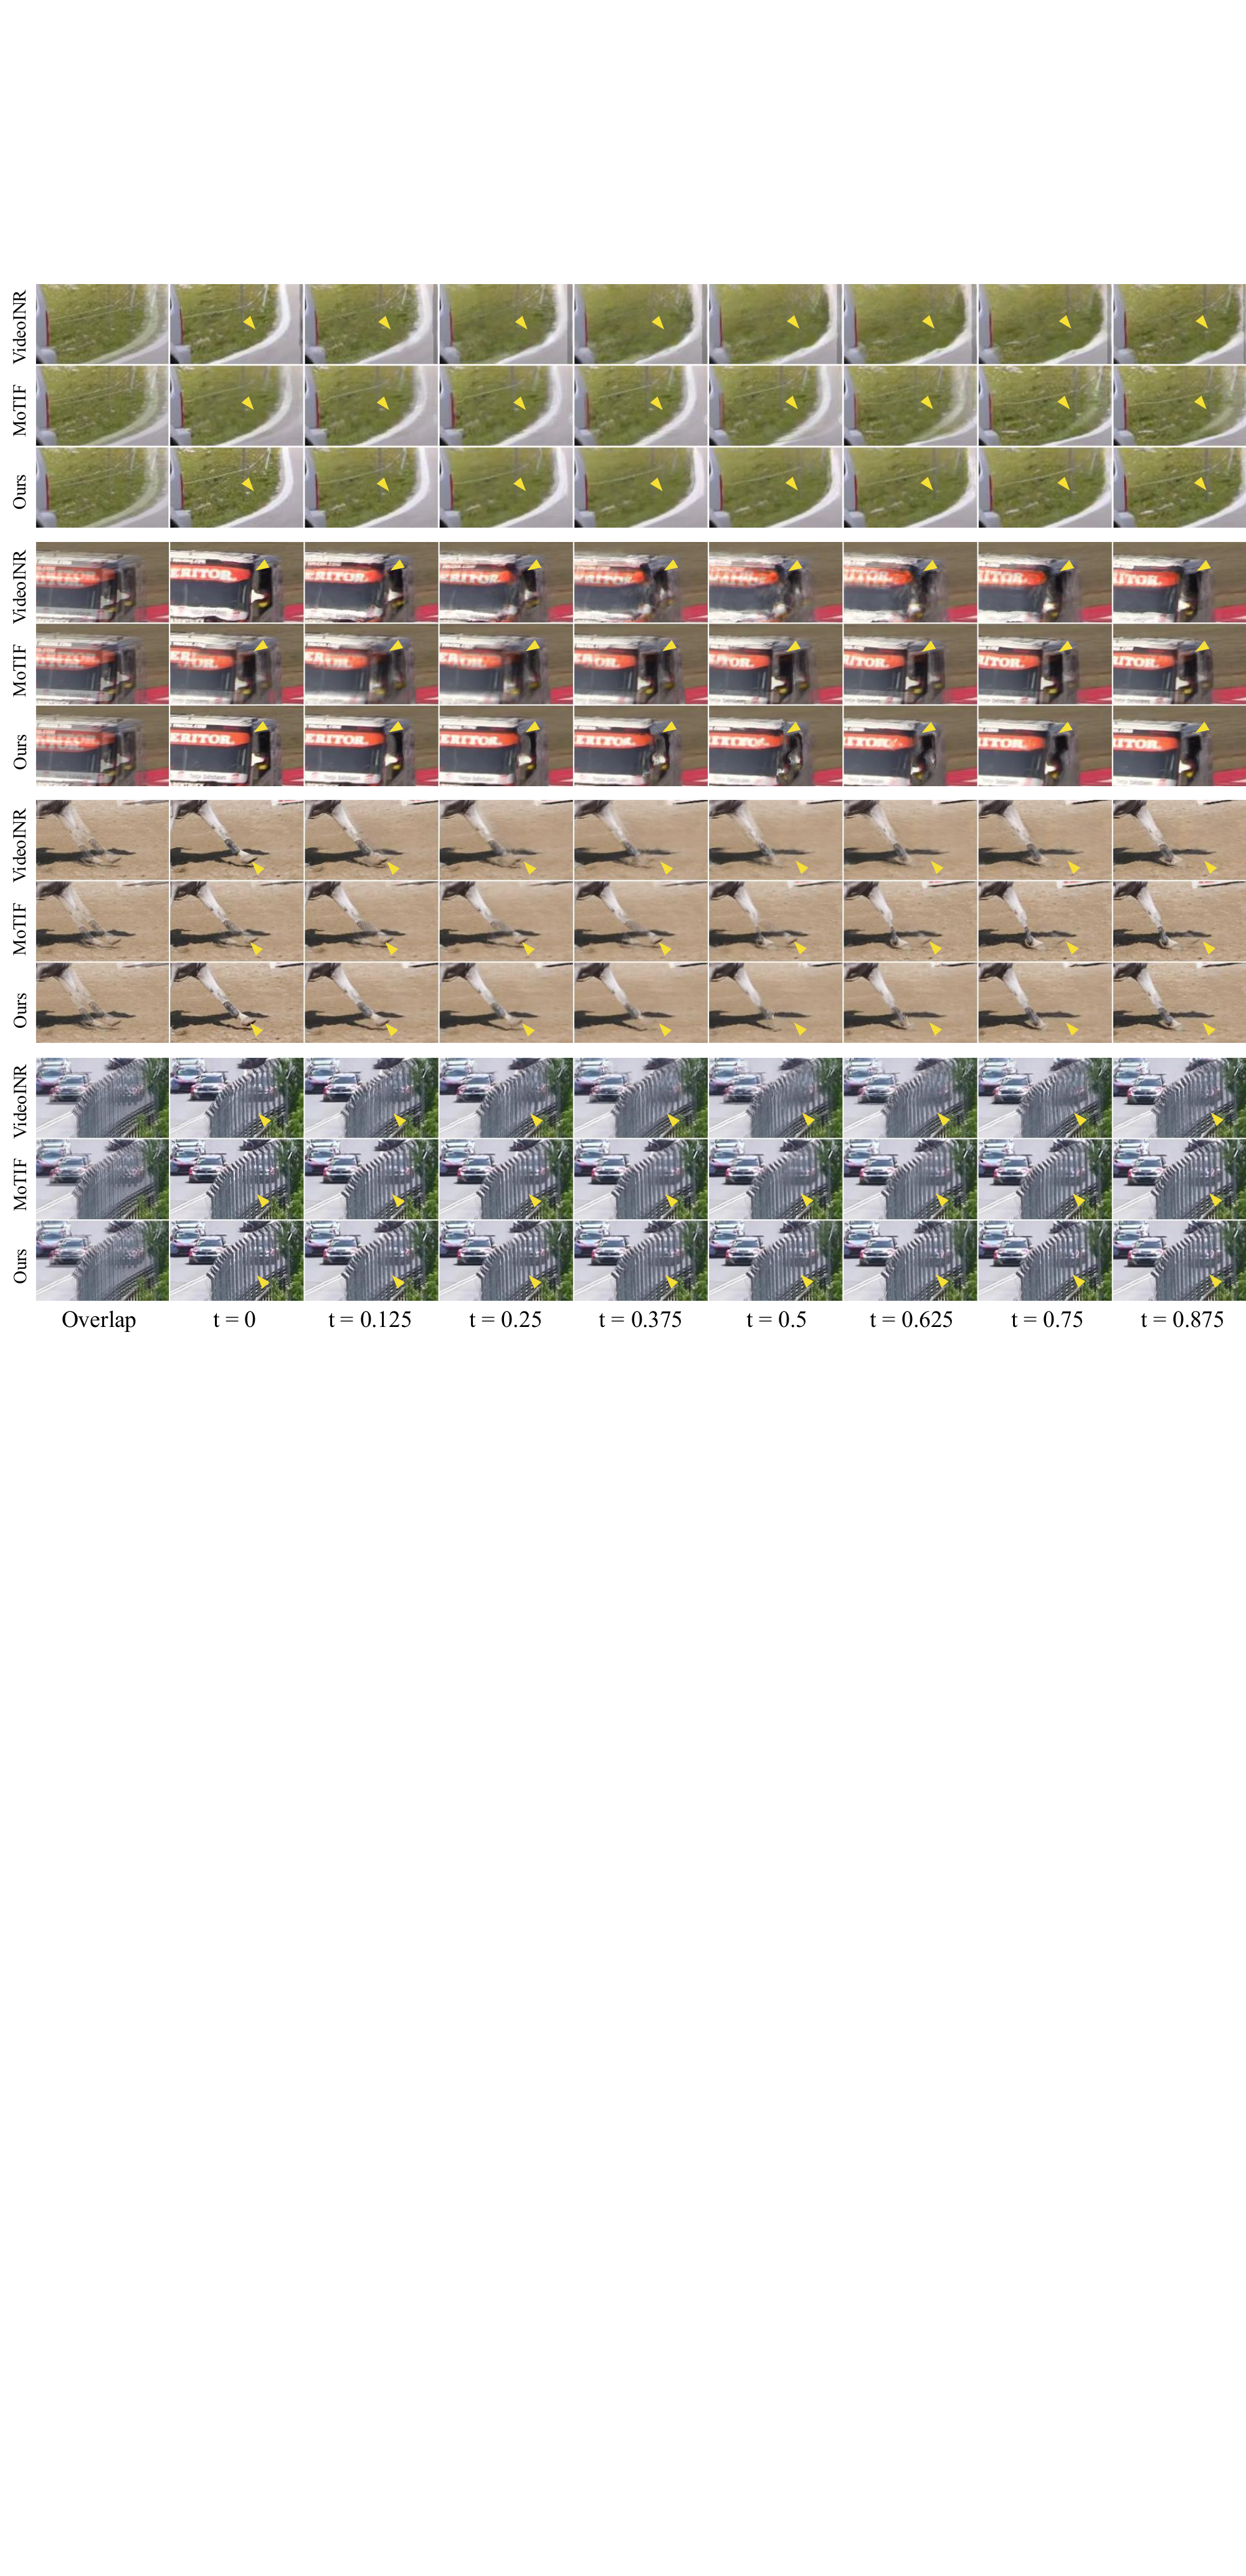}}
    \caption{Qualitative comparison on arbitrary scale temporal interpolation on in-distribution ($\times$8) with all time coordinates. We use the DAVIS dataset for evaluation. ``Overlap'' refers to the averaged image of two input frames ($t=0,1$), and the following images are interpolation results at $t=(0,1)$.  }
    
    \label{figure_x8} 
\end{figure*}
\clearpage
%-------------------------------------------------------------------------

\begin{figure*}[!t]
    \centerline{\includegraphics[width=\linewidth]{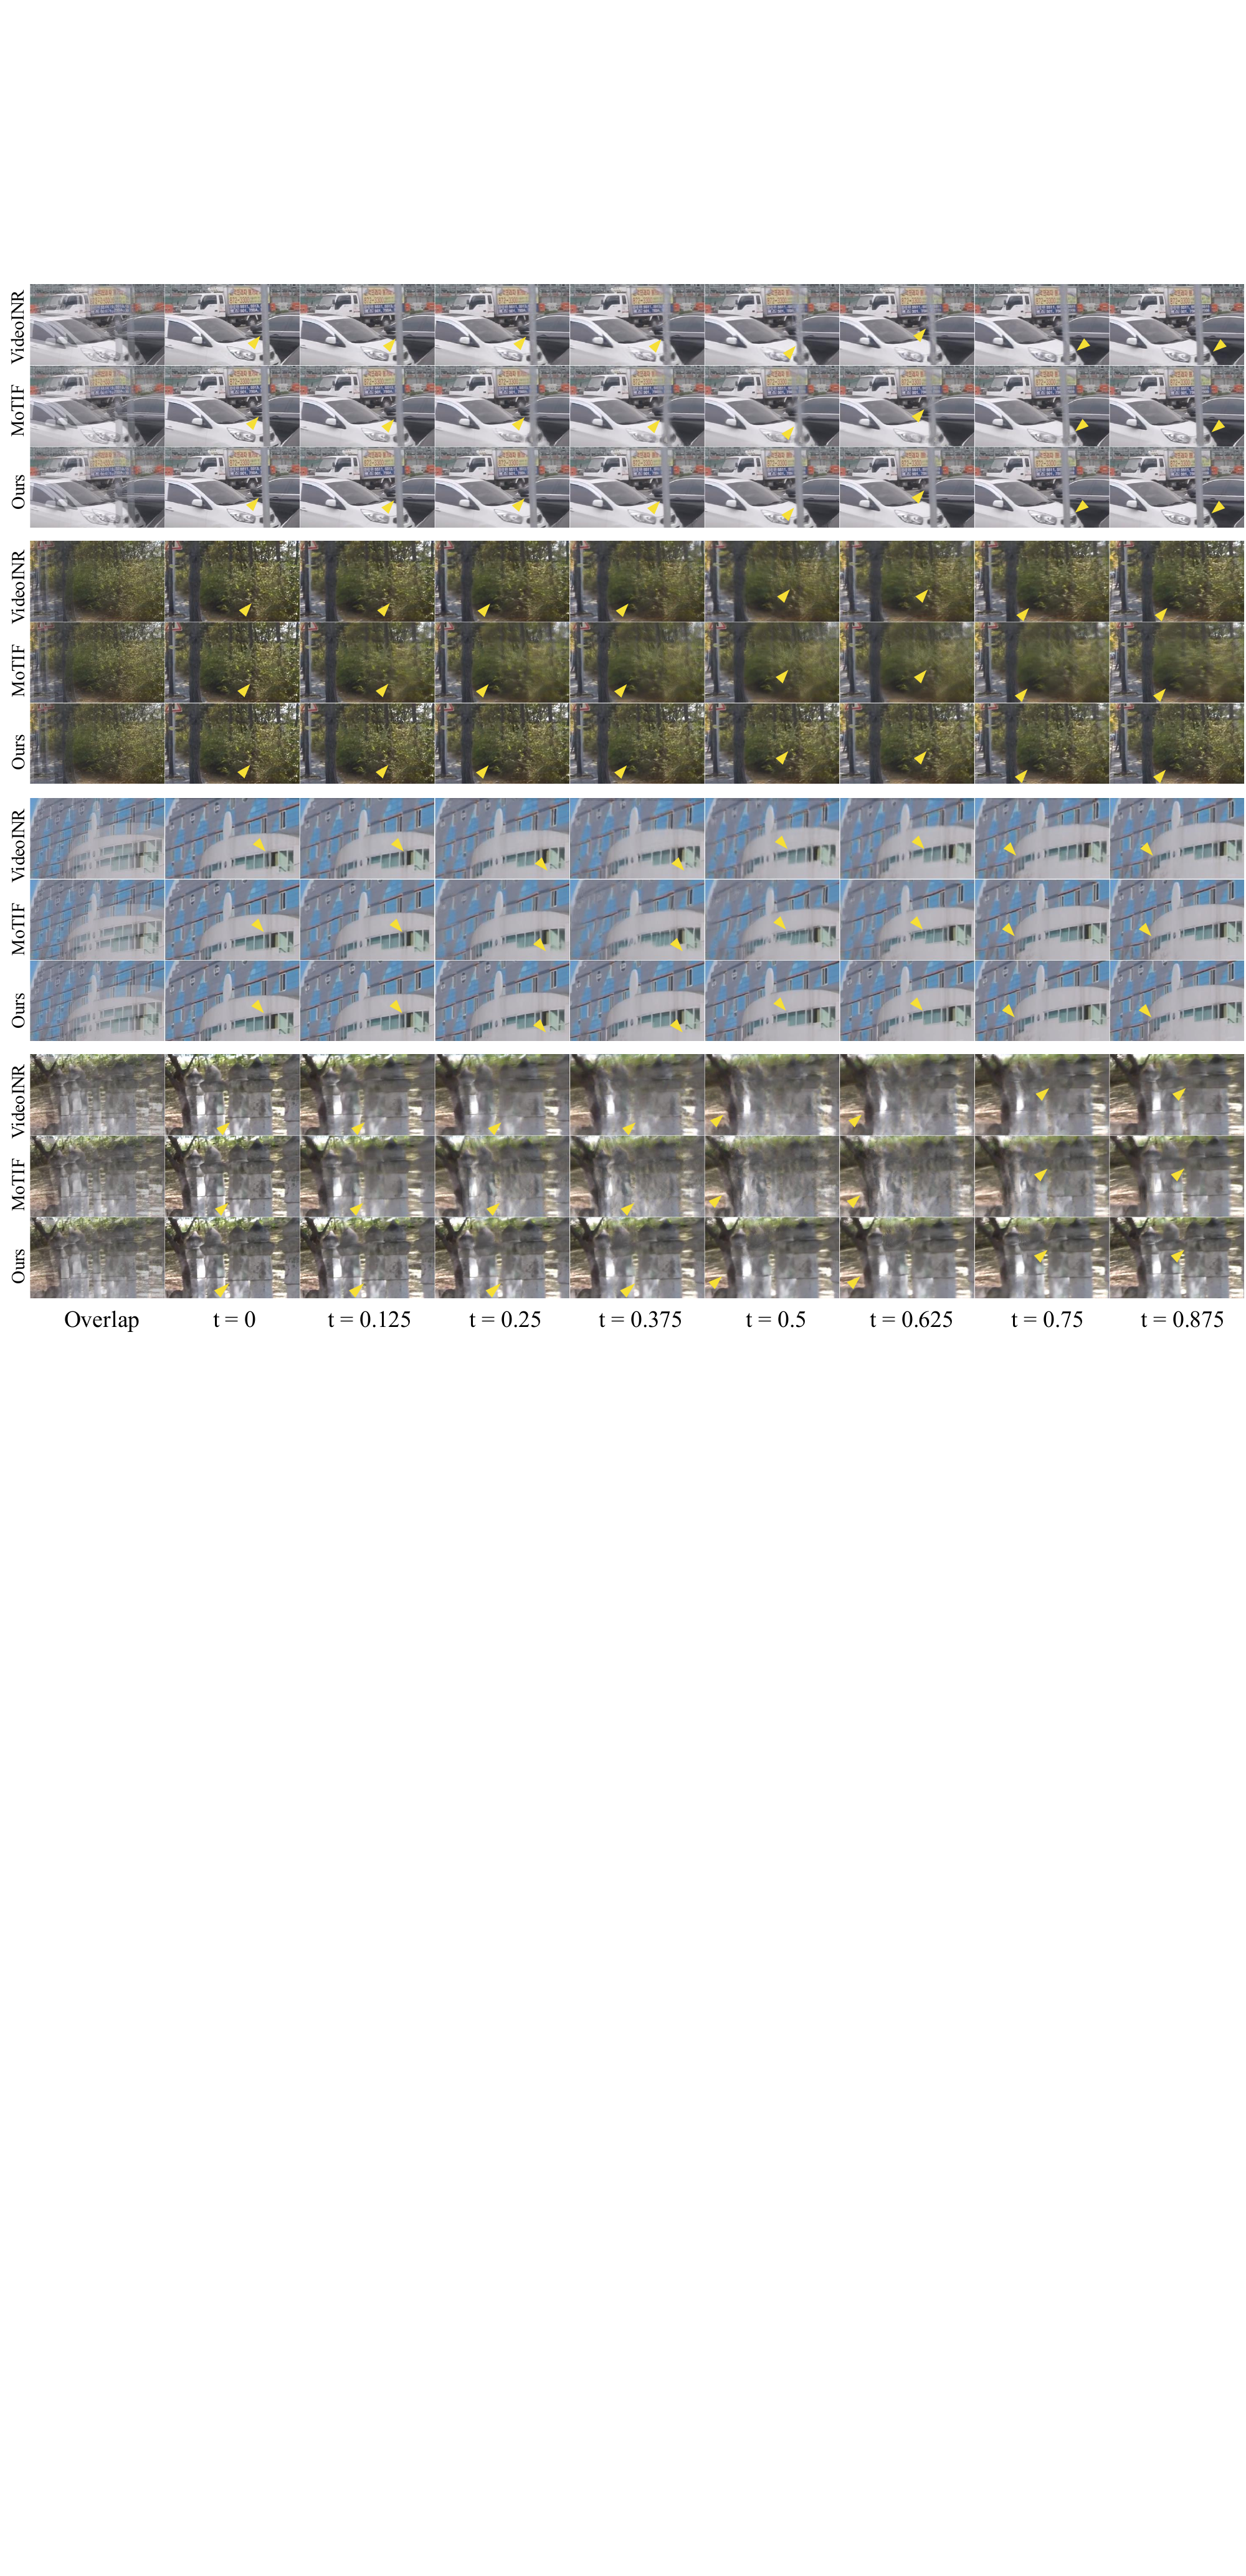}}
    \caption{Qualitative comparison on arbitrary scale temporal interpolation on in-distribution ($\times$8) for temporal scale and in-distribution ($\times$4) for spatial scale with all time coordinates. We use the DAVIS dataset for evaluation. ``Overlap'' refers to the averaged image of two input frames ($t=0,1$), and the following images are interpolation results at $t=(0,1)$.  }
    
    \label{figure_gopro_x4x8} 
\end{figure*}
\clearpage

%-------------------------------------------------------------------------

\begin{figure*}[!t]
    \centerline{\includegraphics[width=\linewidth]{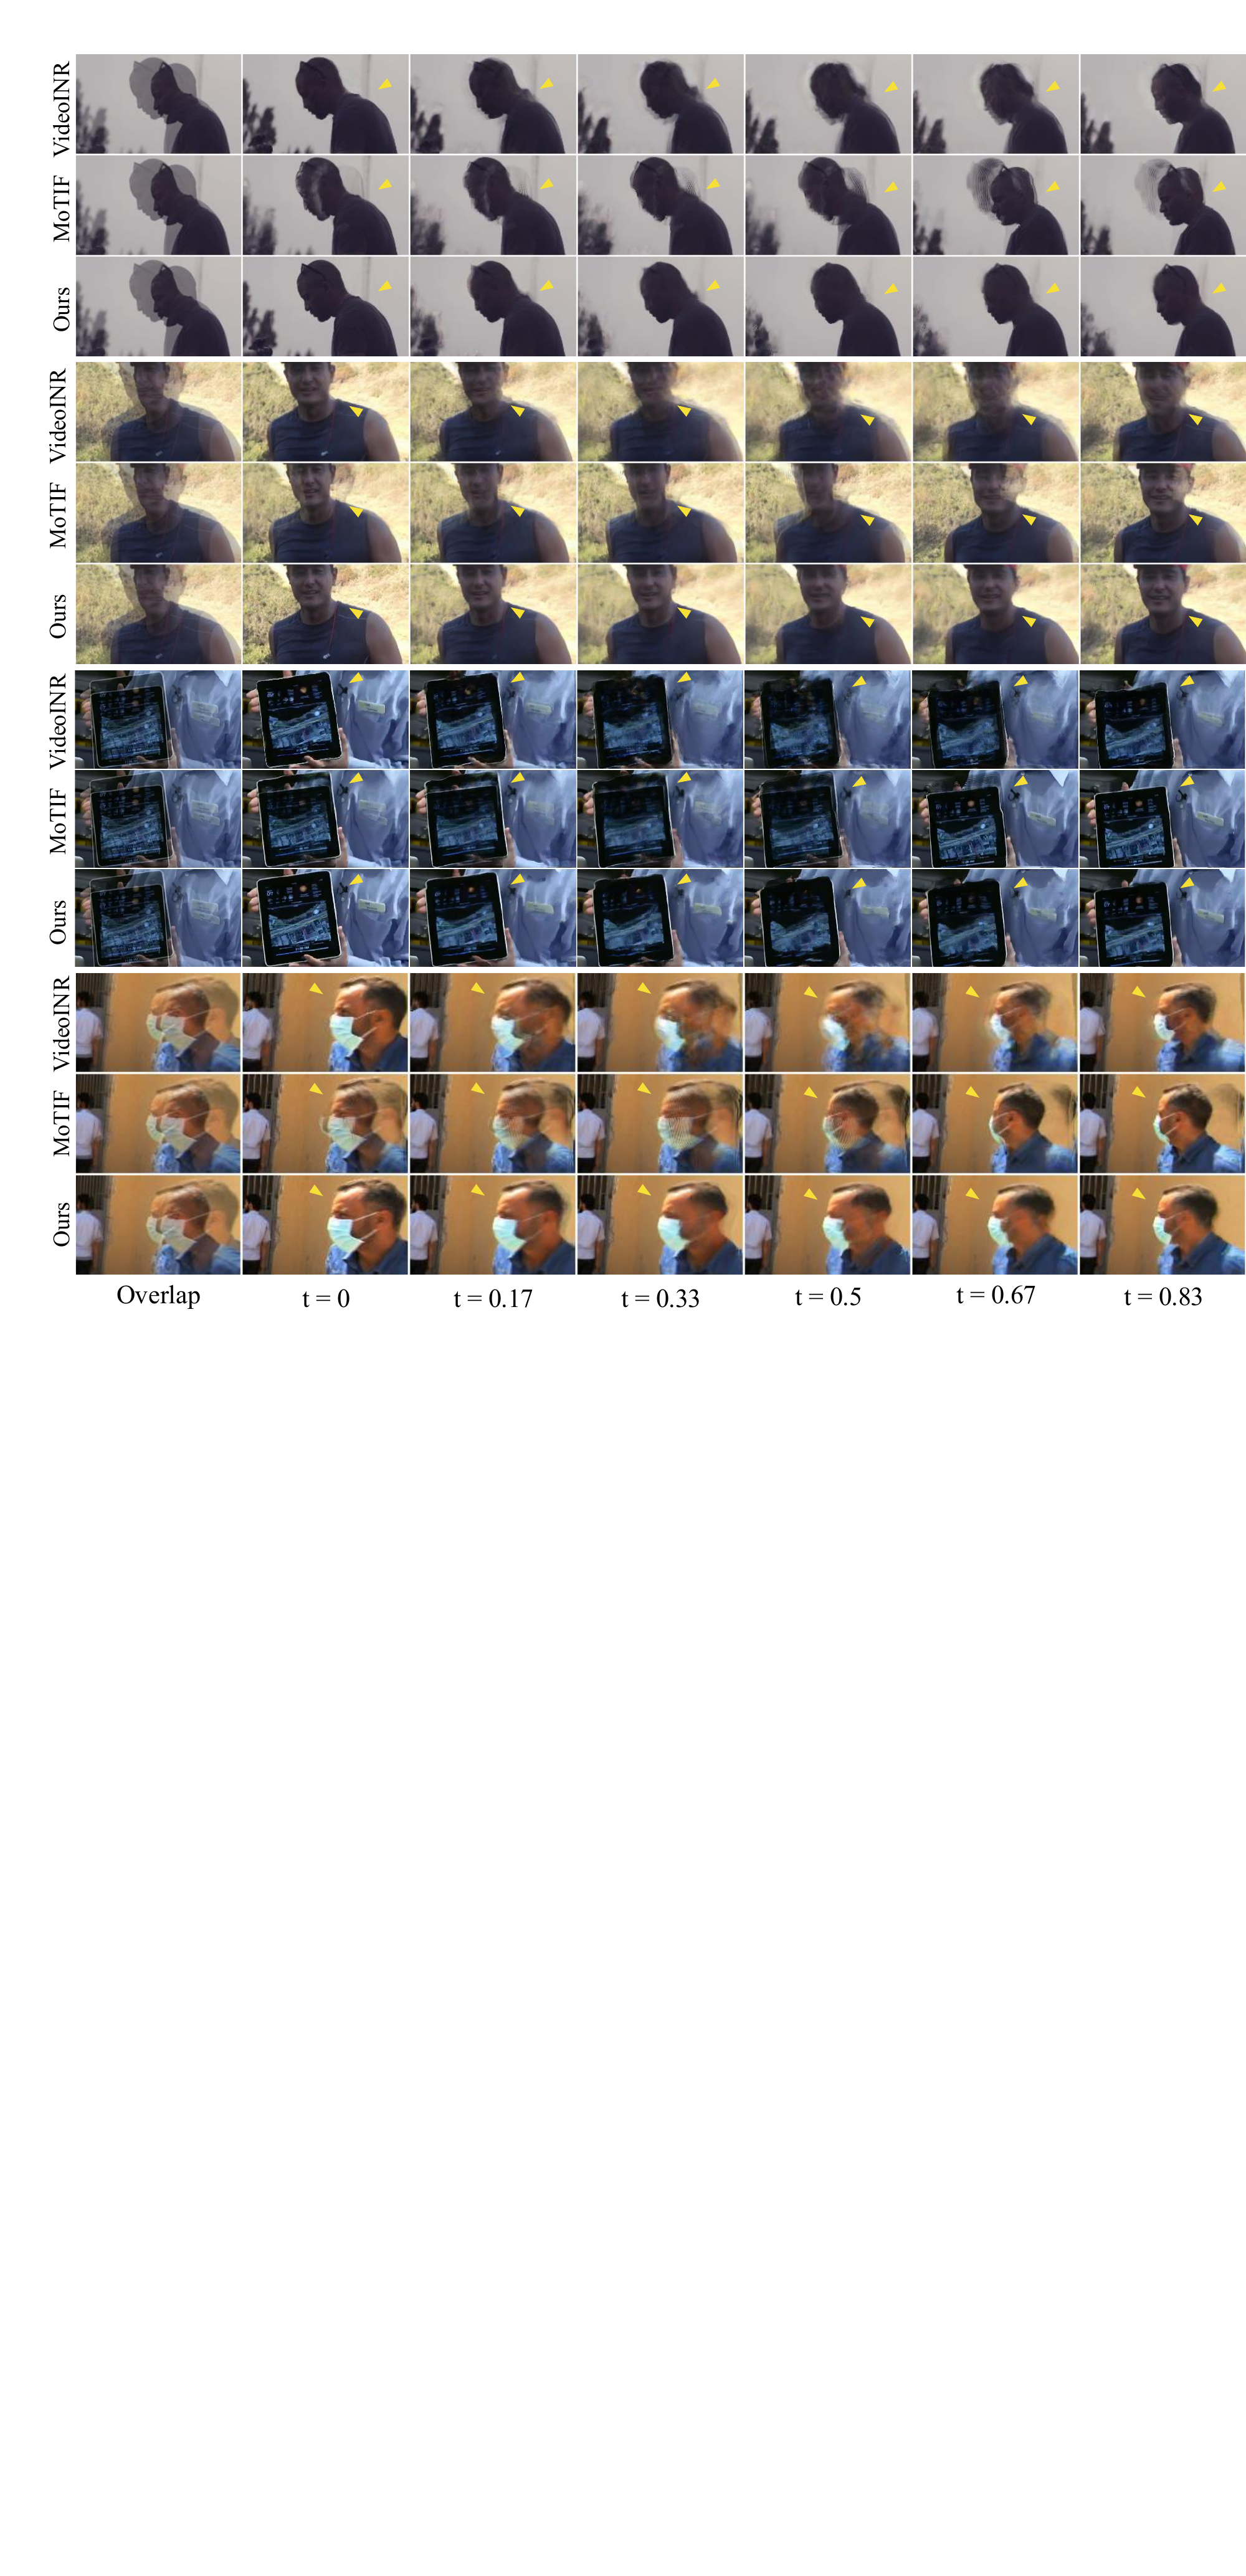}}
    \caption{Qualitative comparison on arbitrary scale temporal interpolation on out-of-distribution ($\times$6) with all time coordinates. We use the Vimeo-medium testset for evaluation. ``Overlap'' refers to the averaged image of two input frames ($t=0,1$), and the following images are interpolation results at $t=(0,1)$.}
    
    \label{figure_vimeo_medium_x1x6} 
\end{figure*}
\clearpage
%-------------------------------------------------------------------------

%-------------------------------------------------------------------------

\begin{figure*}[!t]
    \centerline{\includegraphics[width=\linewidth]{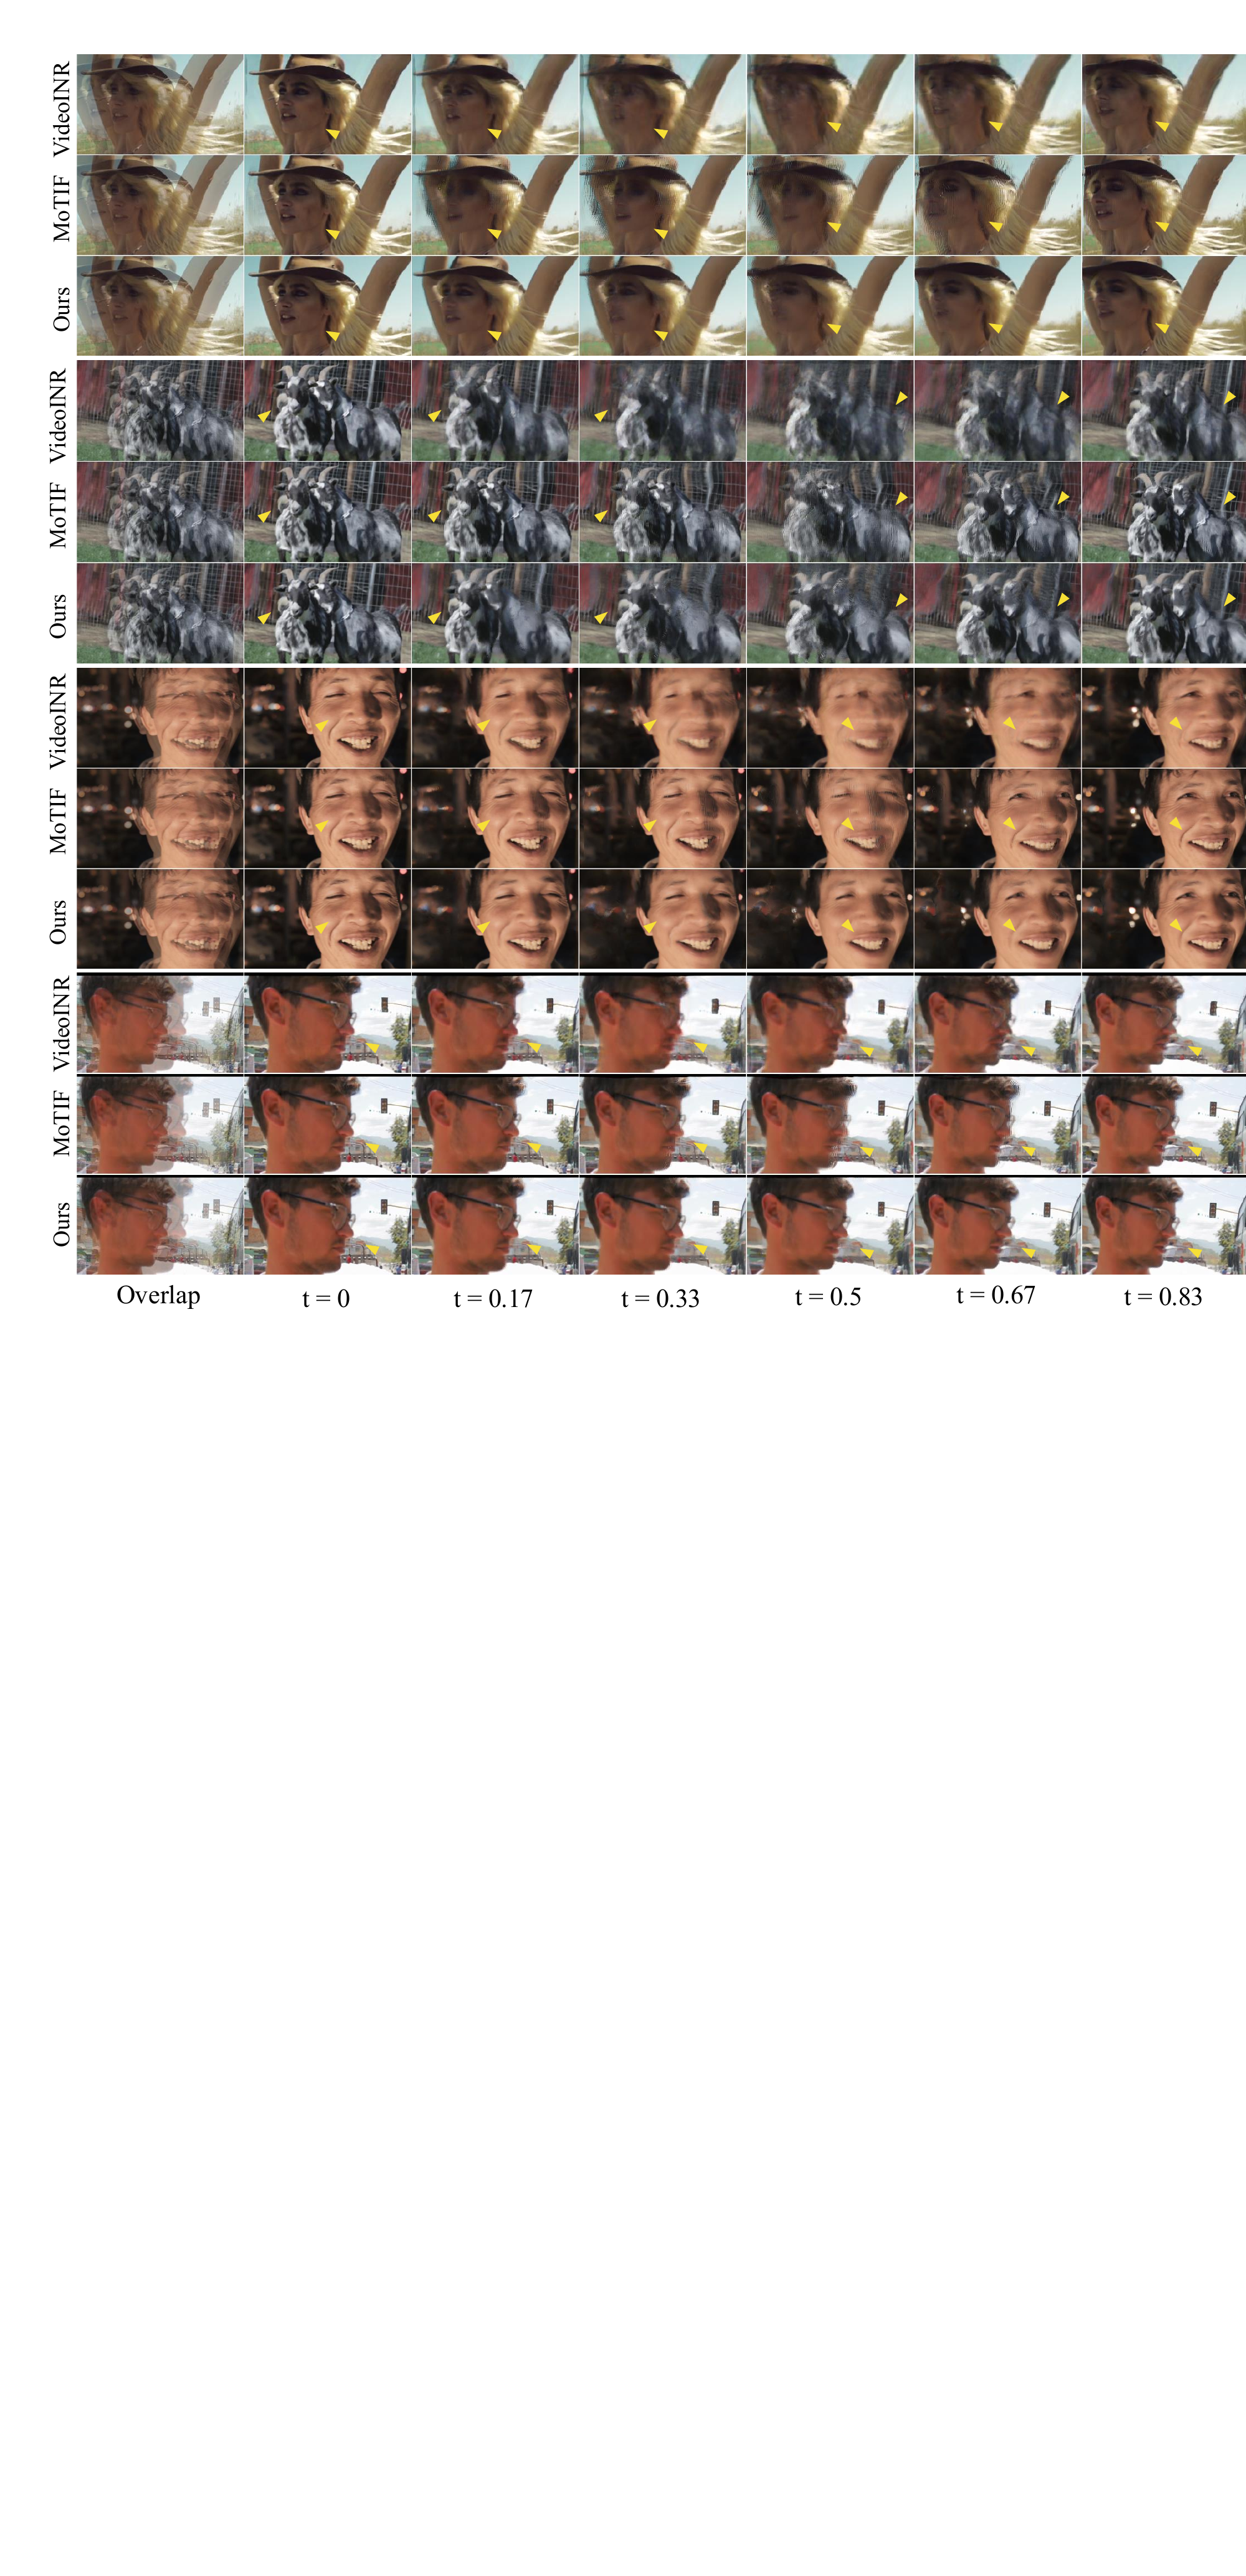}}
    \caption{Qualitative comparison on arbitrary scale spatial-temporal interpolation on out-of-distribution ($\times$6) for temporal scale and out-of-distribution ($\times$2) for spatial scale with all time coordinates. We use the Vimeo-Fast testset for evaluation. ``Overlap'' refers to the averaged image of two input frames ($t=0,1$), and the following images are interpolation results at $t=(0,1)$.}
    
    \label{figure_vimeo_fast_x2x6} 
\end{figure*}
\clearpage
%-------------------------------------------------------------------------

%-------------------------------------------------------------------------

\begin{figure*}[!t]
    \centerline{\includegraphics[width=\linewidth]{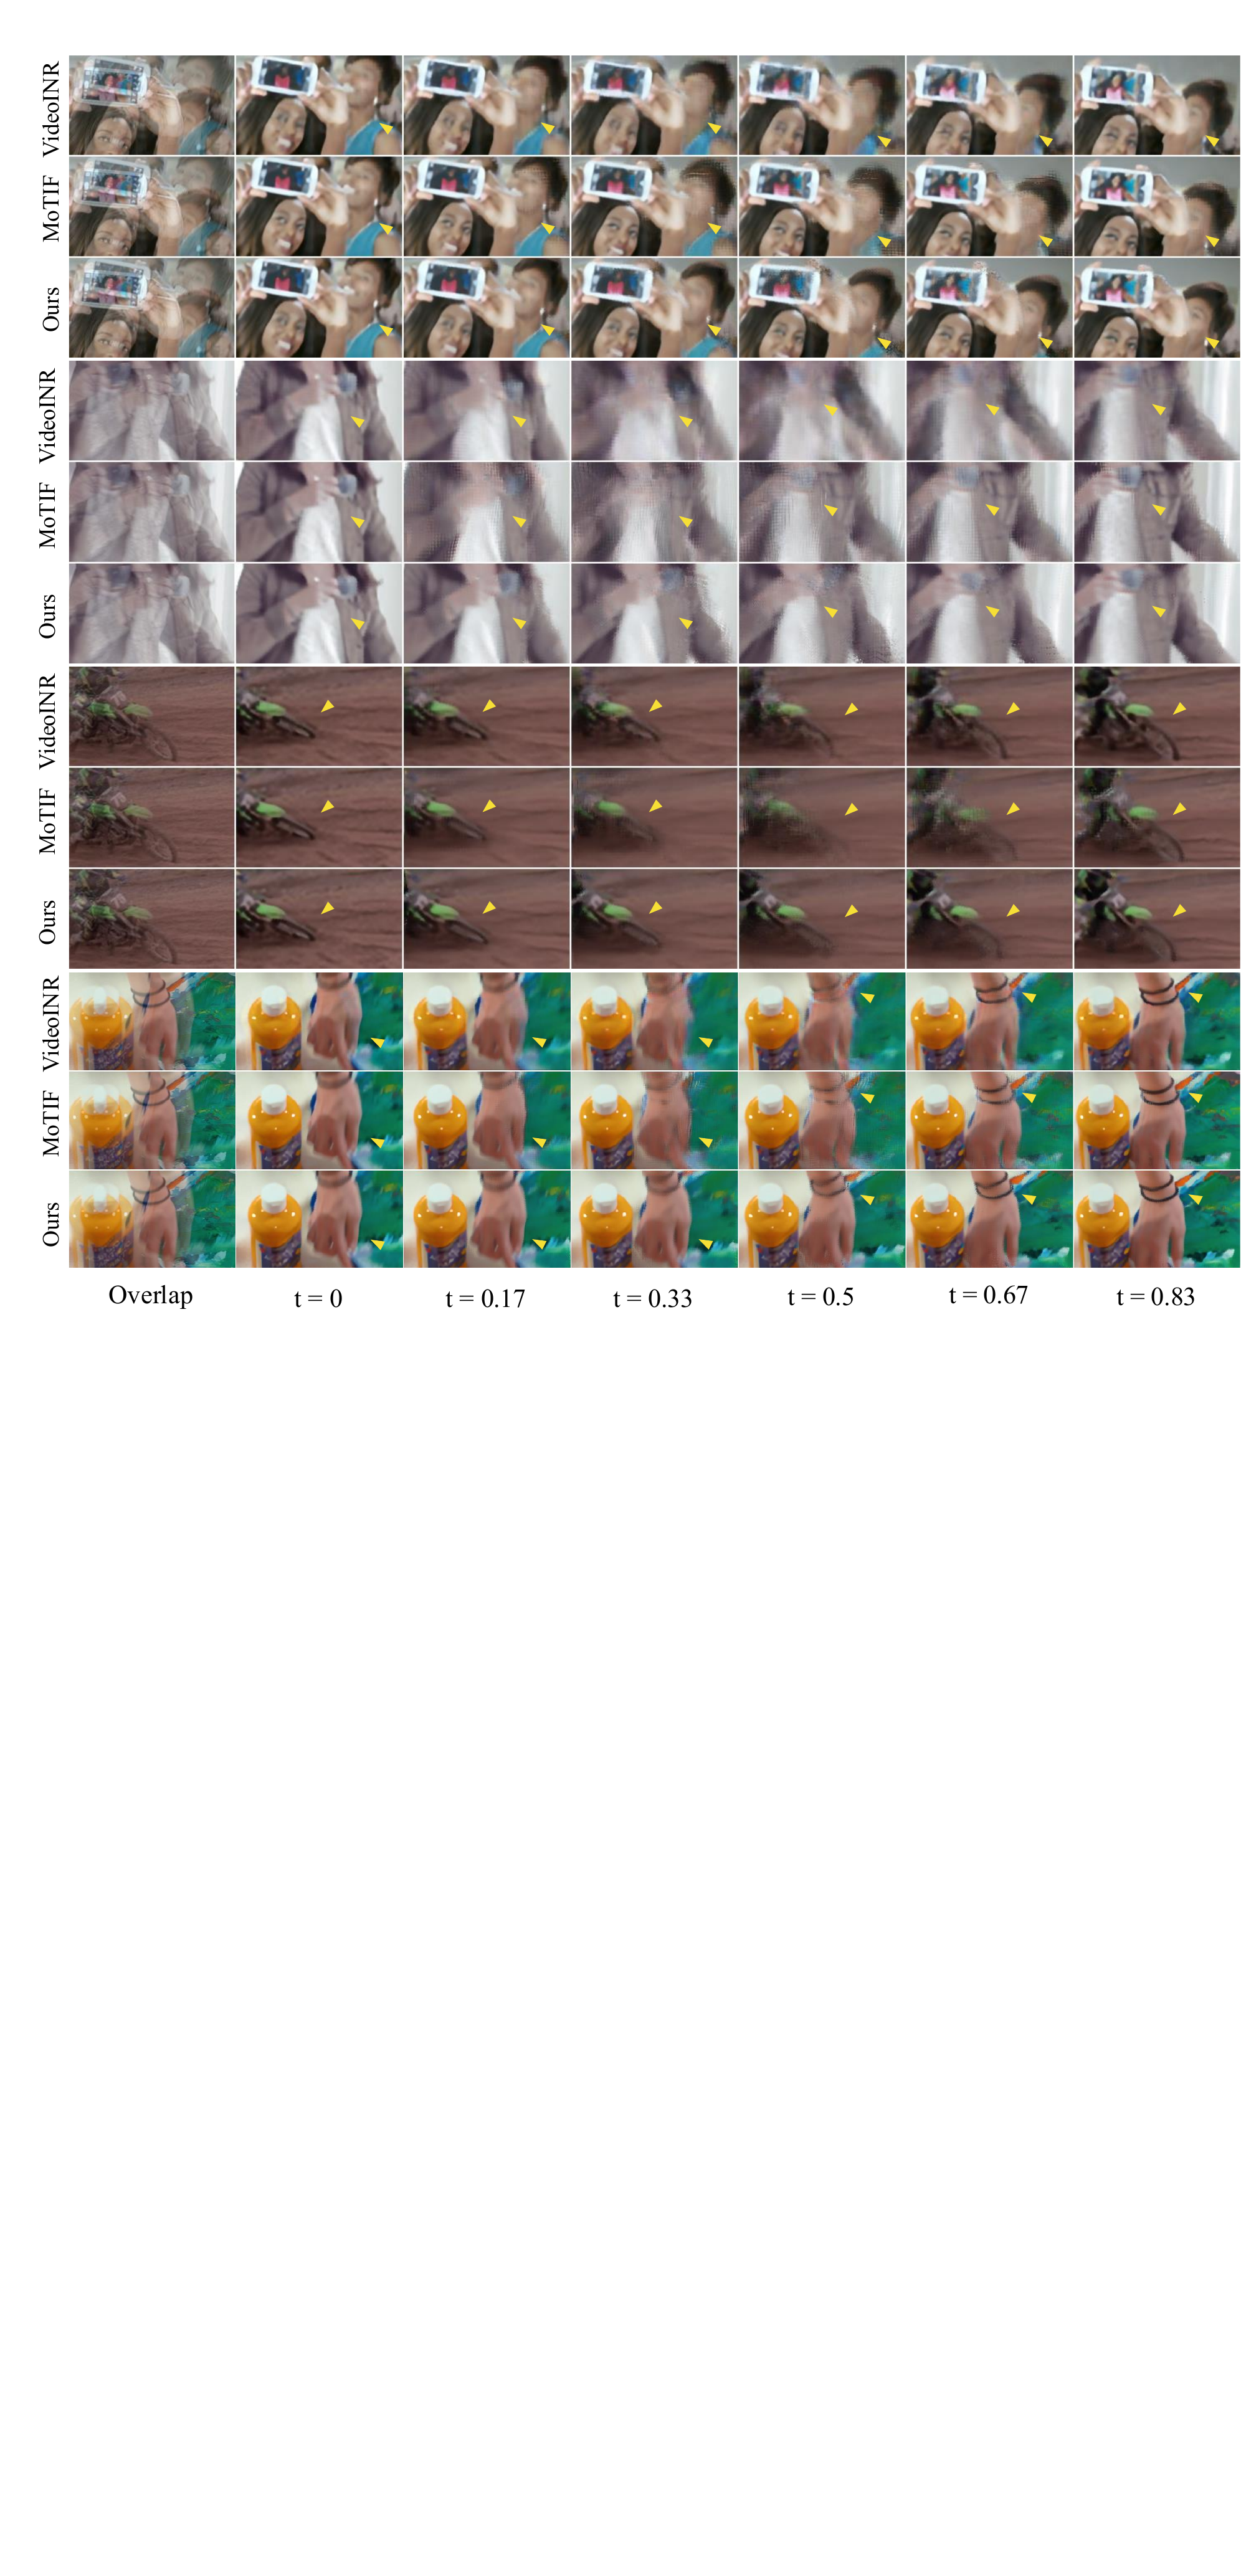}}
    \caption{Qualitative comparison on arbitrary scale spatial-temporal interpolation on out-of-distribution ($\times$6) for temporal scale and out-of-distribution ($\times$4) for spatial scale with all time coordinates. We use the Vimeo-Fast testset for evaluation. ``Overlap'' refers to the averaged image of two input frames ($t=0,1$), and the following images are interpolation results at $t=(0,1)$.}
    
    \label{figure_vimeo_fast_x4x6} 
\end{figure*}
\clearpage
%-------------------------------------------------------------------------
