# Supplementary material for: BF-STVSR: B-Splines and Fourier-Best Friends for High Fidelity Spatial-Temporal Video Super-Resolution
Source: arXiv:2501.11043 source file (2025-03-25)
Supplement: Supplementary file 2 [file X_suppl.tex]

\clearpage
\setcounter{page}{1}
\maketitlesupplementary

%-------------------------------------------------------------------------

\begin{figure*}[!ht]
    \centerline{\includegraphics[width=\linewidth]{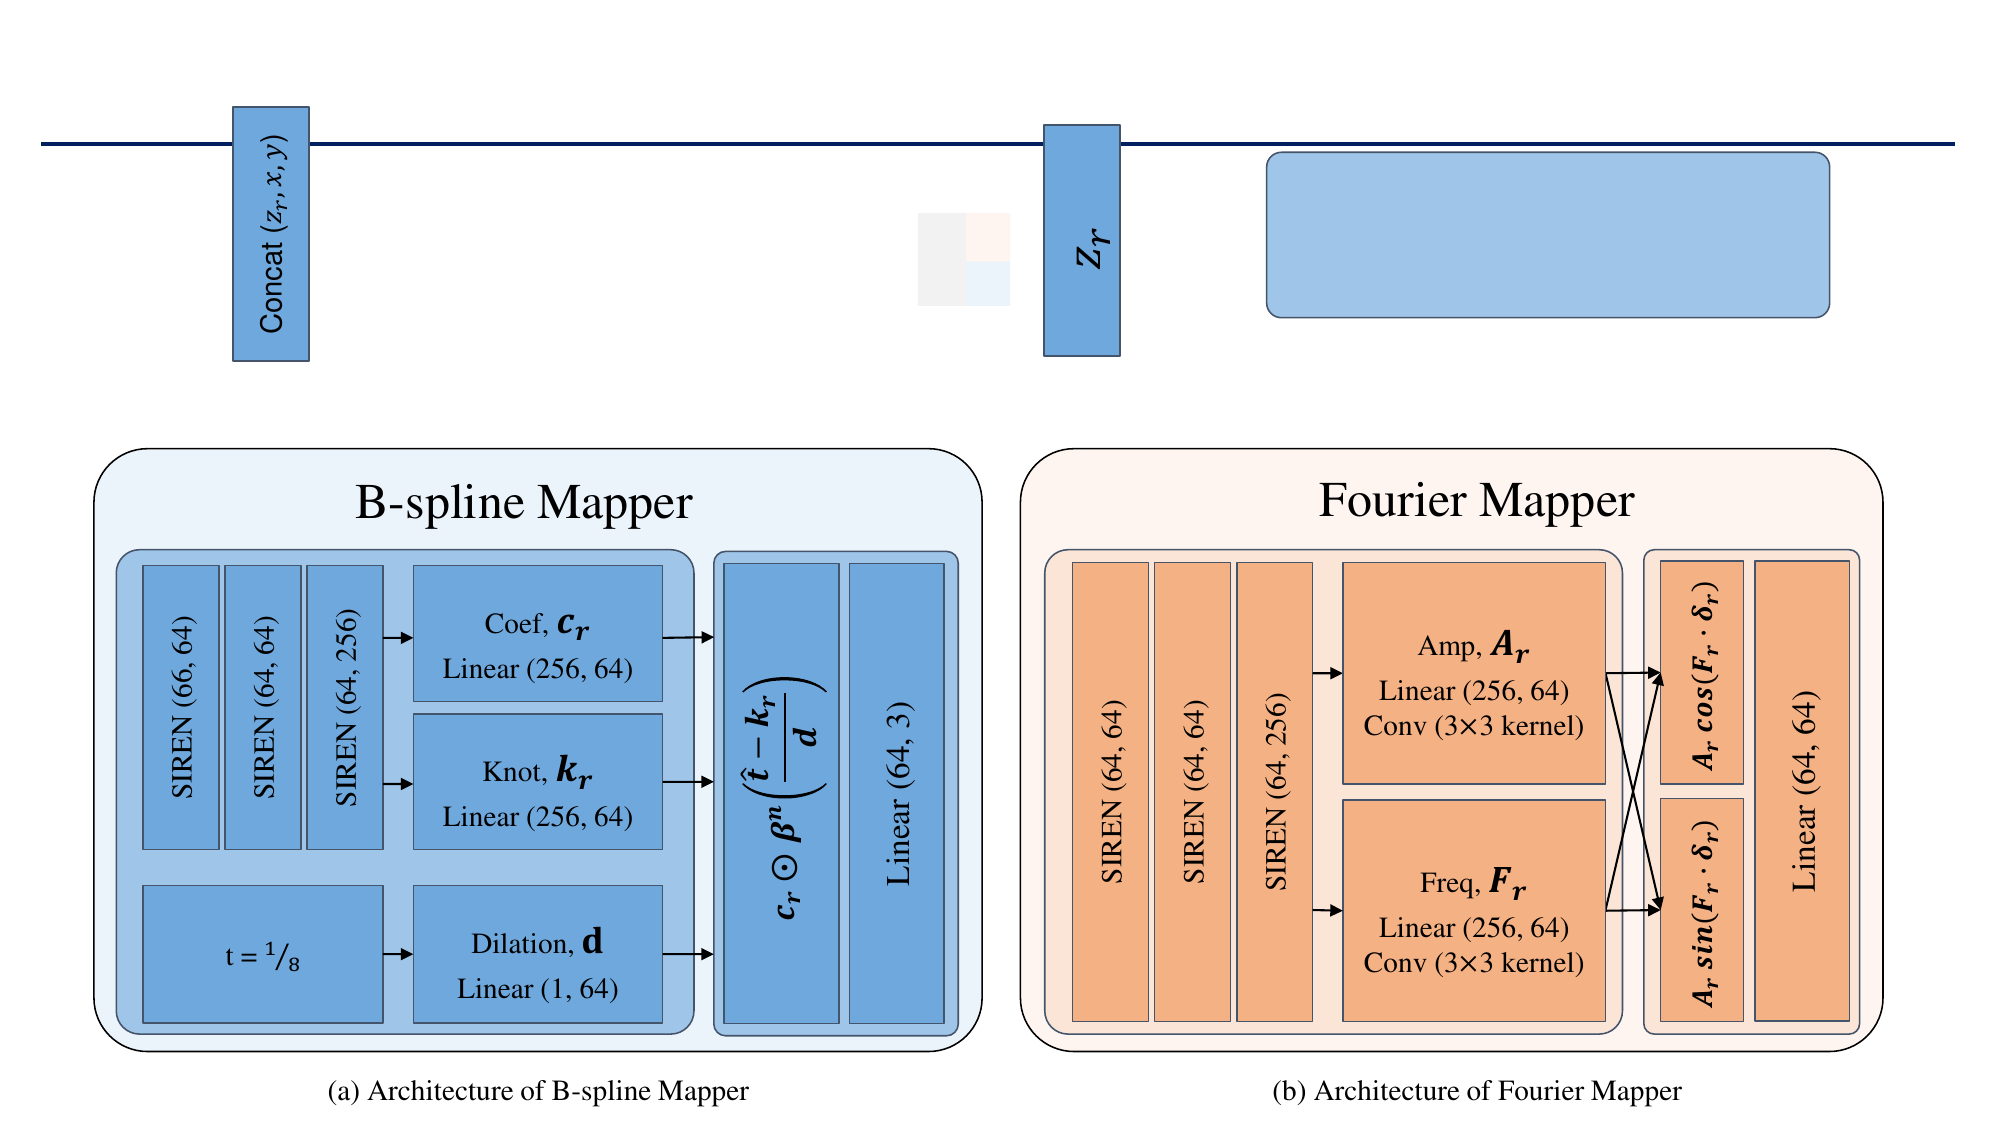}}
    \caption{Detailed Architectures of of {\bspline} and {\fourier}. }
    
    \label{fig_mappers} 
\end{figure*}

%-------------------------------------------------------------------------

\begin{table*}[t!]
\centering
\caption{Performance comparison on the C-STVSR baselines on Vimeo90K dataset. Results are evaluated using PSNR (dB) and SSIM metrics. All frames are interpolated by a factor of $\times 4$ in the spatial axis and $\times 6$ in the temporal axis. \textbf{Bold} indicates the best performance.}
\label{tab:table1}
% \resizebox{0.8\textwidth}{!}{%
\begin{tabular}{c|ccc}
\hline
\multirow{2}{*}{Method}  & \multicolumn{3}{c}{Test Dataset} \\ 
% \hline
\cline{2-4}
 & Vimeo-\texttt{Fast} & Vimeo-\texttt{Medium} & Vimeo-\texttt{Slow} \\ 
\hline
\hline
 VideoINR \cite{chen2022vinr} & 25.79 / 0.7980 & 28.37 / 0.8553 & 29.25 / 0.8727 \\

 MoTIF \cite{chen2023motif} & 26.03 / 0.7909 & 28.68 / 0.8574 & 29.47 / 0.8739 \\

 Ours & \textbf{26.53 / 0.8079}  & \textbf{28.76 / 0.8594} & \textbf{29.53 / 0.8748} \\
\hline

\end{tabular}%
% }
\end{table*}

%-------------------------------------------------------------------------

\begin{table*}[t!]
\centering
\caption{Performance comparison on the C-STVSR baselines on on Gopro, and Adobe240 datasets. Baseline models are trained on Vimeo90K septuplet dataset. Results are evaluated using PSNR (dB) and SSIM metrics. All frames are interpolated by a factor of $\times 4$ in the spatial axis and $\times 8$ in the temporal axis. \textbf{Bold} indicates the best performance.}
\label{tab:table2}
% \resizebox{0.8\textwidth}{!}{%
\begin{tabular}{c|cccc}
\hline
\multirow{2}{*}{Method}  & \multicolumn{4}{c}{Test Dataset} \\ 
% \hline
\cline{2-5}
 & Adobe-\textit{Average} & Adobe-\textit{Center}  & Gopro-\textit{Average} & Gopro-\textit{Center} \\ 
\hline
\hline
 VideoINR \cite{chen2022vinr} & 28.95 / 0.8527 & 29.58 / 0.8603 & 29.43 / 0.8657 & 30.20 /  0.8751 \\

 MoTIF \cite{chen2023motif} &  28.81 / 0.8495 & 29.47 / 0.8580 & 29.44 / 0.8649 & 30.24 / 0.8742 \\

 Ours & \textbf{29.30 / 0.8611}  & \textbf{29.88 / 0.8677} & \textbf{29.75 / 0.8709} & \textbf{30.53 / 0.8796} \\
\hline

% 450000
% \multirow{3}{*}{Vimeo}  & VideoINR \cite{chen2022vinr} & 27.35 / 0.8256  & 29.16 / 0.8637 & 29.99 / 0.8792 \\

%   & MoTIF \cite{chen2023motif} & 26.78 / 0.8086  & 28.92 / 0.8584 & 29.68 / 0.8725 \\

%   & Ours & - / -  & - / - & - / - \\

% 400000
% \multirow{3}{*}{Vimeo}  & VideoINR \cite{chen2022vinr} & 27.13 / 0.8215  & 29.04 / 0.8614 & \textbf{29.88} / 0.8769 \\

%   & MoTIF \cite{chen2023motif} & 26.60 / 0.8050  & 28.83 / 0.8570 & 29.60 / 0.8714 \\

%   & Ours & \textbf{27.20 / 0.8227}  & \textbf{29.09 / 0.8626} & 29.85 / \textbf{0.8774} \\

% \hline

\end{tabular}%
% }
\end{table*}

%-------------------------------------------------------------------------

\section{Definition of B-spline function}

The B-spline basis function $\beta^n(x)$ is defined as the $n$-fold convolution of $\beta^0(x)$ with itself, where $n$ represents the polynomial degree. The function $\beta^0(x)$ equals 1 when $\vert x\vert < 0.5$ and 0 otherwise. As $n$ increases, the support expands: $\beta^1(x)$ spans $[-1, 1]$, $\beta^2(x)$ spans $[-1.5, 1.5]$, and $\beta^3(x)$ spans $[-2, 2]$. In this study, we adopt the third-order B-spline ($n = 3$) for {\bspline}. The definitions of $\beta^3(x)$ and its derivative $\frac{\partial}{\partial x} \beta^3(x)$ are provided in \Eref{eq:b-spline} and \Eref{eq:b-spline-back}, respectively.

% The B-spline basis function $\beta^n(x)$ is defined by recursively convolving $\beta^0(x)$ with itself $n$ times, where $n$ is the polynomial degree. The function $\beta^0(x)=1$ for $\vert x\vert <0.5$ and $\beta^0(x)=0$ otherwise. As $n$ increases, the support widens: $\beta^1(x)$ spans $[-1,1]$, $\beta^2(x)$ spans $[-1.5, 1.5]$ and $\beta^3(x)$ spans $[-2,2]$. In this study, we use third-order B-spline (n=3) for {\bspline}. We provide definition of $\beta^3(x)$ in \Eref{eq:b-spline} and differentiated $\frac{\partial}{\partial x} \beta^3(x)$  in \Eref{eq:b-spline-back}.

% In this study, we use a third-order B-spline (n=3) for {\bspline}. The definition of B-spline function and The $\beta^0(x)$ is 1 if $\left\vert x \right\vert < 0.5$ and 0 if otherwise. The $\beta^1(x)$ is $1-\left\vert x \right\vert$ if $\left\vert x \right\vert \leq 1$ and 0 if otherwise. Here, we use third-order $\beta^3(x)$ as our basis function and the definition is like \ref{eq:b-spline}, the backpropagation of it is in \ref{eq:b-spline-back}.

\begin{equation} \label{eq:b-spline}
\beta^3(x) =
\begin{cases} 
\frac{1}{6}(2 + x)^3 & \text{if } -2 < x \leq -1; \\
\frac{1}{6}(4 - 6x^2 - 3x^3) & \text{if } -1 < x \leq 0; \\
\frac{1}{6}(4 - 6x^2 + 3x^3) & \text{if } 0 < x \leq 1; \\
\frac{1}{6}(2 - x)^3 & \text{if } 1 < x \leq 2; \\
0 & \text{otherwise}.
\end{cases}
\end{equation}
\begin{equation} \label{eq:b-spline-back}
\frac{\partial}{\partial x} \beta^3(x) =
\begin{cases} 
\frac{1}{2}(2 + x)^2 & \text{if } -2 < x \leq -1; \\
-2x - 1.5x^2 & \text{if } -1 < x \leq 0; \\
-2x + 1.5x^2 & \text{if } 0 < x \leq 1; \\
-\frac{1}{2}(2 - x)^2 & \text{if } 1 < x \leq 2; \\
0 & \text{otherwise}.
\end{cases}
\end{equation}

\section{Detailed Architectures of Mappers}
We present the detailed network architecture of {\bspline} and {\fourier} in \Fref{fig_mappers}. Both mappers take encoder features as input and capture temporal/spatial information using three-layer SIRENs \cite{siren}. In {\bspline}, a linear layer is used for each coefficient estimator, predicting the coefficients, knots, and dilations for B-spline representations. In {\fourier}, linear and convolutional layers follow the SIREN layers to estimate the amplitudes and frequencies of the Fourier coefficients. Finally, the B-spline or Fourier representations are passed through a linear layer to produce motion vectors or spatial features.

\section{Additional Results on Vimeo90K}

We further evaluate existing C-STVSR models, including VideoINR \cite{chen2022vinr}, MoTIF \cite{chen2023motif}, and BF-STVSR, all trained on the Adobe240fps dataset, using the Vimeo90K dataset. Vimeo90K, a widely used benchmark for video enhancement, comprises 64,612 clips, each containing seven frames. Following \cite{xiang2020zooming}, we categorize the test set into three motion groups: \texttt{Fast}, \texttt{Medium}, and \texttt{Slow}. The evaluation results, presented in \Tref{tab:table1}, show that our model achieves higher PSNR across all motion categories compared to other methods. Notably, it outperforms VideoINR by approximately 0.7 dB and MoTIF by 0.5 dB on the Vimeo-\texttt{Fast} subset, highlighting its superior ability to effectively handle motion dynamics, even in challenging scenarios.

Additionally, we train the C-STVSR models (VideoINR, MoTIF, and BF-STVSR) using the Vimeo90K training set. Similar to the Adobe240fps dataset, we select seven consecutive frames from each video clip, use the $1^{st}$ and $7^{th}$ frames as input reference frames, and randomly sample three intermediate frames as ground-truth targets. These models are then evaluated on the GoPro and Adobe240fps datasets, following the \textit{-Center} and \textit{-Average} evaluation protocols detailed in the main paper. The results, presented in \Tref{tab:table2}, demonstrate that our model consistently achieves higher PSNR across all datasets, with improvements of approximately 0.4 dB over VideoINR and 0.3 dB over MoTIF.

These results suggest that our model is both robust and versatile. While trained on specific datasets, it shows promising generalization across diverse datasets, achieving competitive performance in reconstructing high-quality frames. In comparison, previous methods exhibit some challenges in adapting to unseen data, highlighting the potential advantages of our approach.

% Vimeo90K \cite{xue2019video} is one of the most widely used dataset for video enhancement task, consisting of 64,612 clips, each containing 7 frames. We evaluate the existing C-STVSR models, including VideoINR \cite{chen2022vinr}, MoTIF \cite{chen2023motif}, and BF-STVSR, on the Vimeo90K septuplet testset. Following \cite{xiang2020zooming}, we divide the testset into three subsets based on motion: \texttt{Fast}, \texttt{Medium}, and \texttt{Slow} motion. The evaluation results are presented in the first row of \Tref{tab:table1}. Our model achieves the best performance across all motion categories, with notable improvement of approximately 0.5dB over MoTIF on the Vimeo-Fast subset. This demonstrates the effectiveness of our model in capturing dynamic motion compared to existing C-STVSR approaches.

% Additionally, We train the existing C-STVSR models, VideoINR, MoTIF and BF-STVSR, with Vimeo90K septuplet trainset. Similarly with Adobe240fps dataset, during training, seven sequential frames in the video clip are selected and the $1^{st}$ and $7^{th}$ frames are used as input reference frames. Three frames are then randomly sampled between them and used as the target ground-truth frames. For evaluation, we use Vimeo90K septuplet testset. We show the evaluation results in second row of \Tref{tab:table1}.

\section{Additional Qualitative Results}

We provide more qualitative comparison between BF-STVSR and prior methods (VideoINR \cite{chen2022vinr}, MoTIF \cite{chen2023motif}), all trained on the Adobe240fps dataset. \Fref{figure_x6} and \Fref{figure_x8} present temporal interpolation results (with the spatial scale fixed at 1) on the DAVIS dataset across all temporal coordinates, which were not shown in the main paper, at both the out-of-distribution scale ($\times 6$) and in-distribution scale ($\times 8$), respectively. \Fref{figure_gopro_x4x8} shows the spatio-temporal interpolation results on the GoPro dataset at in-distribution temporal scale ($\times 8$) and in-distribution spatial scale ($\times 4$). \Fref{figure_vimeo_medium_x1x6} shows the temporal interpolation results on the Vimeo-\texttt{Medium} test set at the out-of-distribution scale ($\times 6$). \Fref{figure_vimeo_fast_x2x6} and \Fref{figure_vimeo_fast_x4x6} show spatio-temporal interpolation results on the Vimeo-\texttt{Fast} test set at the out-of-distribution temporal scale ($\times 6$) and both out-of-distribution and in-distribution spatial scales ($\times 2$, $\times 4$), respectively. Additionally, we provide the interpolated video results in supplementary file.

{
    \small
    \bibliographystyle{ieeenat_fullname}
    \bibliography{suppl}
}

%-------------------------------------------------------------------------

%-------------------------------------------------------------------------

% %-------------------------------------------------------------------------
% \begin{figure}[p]
% \centering
% \includegraphics[width=\textwidth]{your-image-file.png} % Replace with your file name
% \caption{Your caption here.}
% \label{fig:your-label}
% \end{figure}
% \clearpage

\begin{figure*}[!t]
    \centerline{\includegraphics[width=\linewidth]{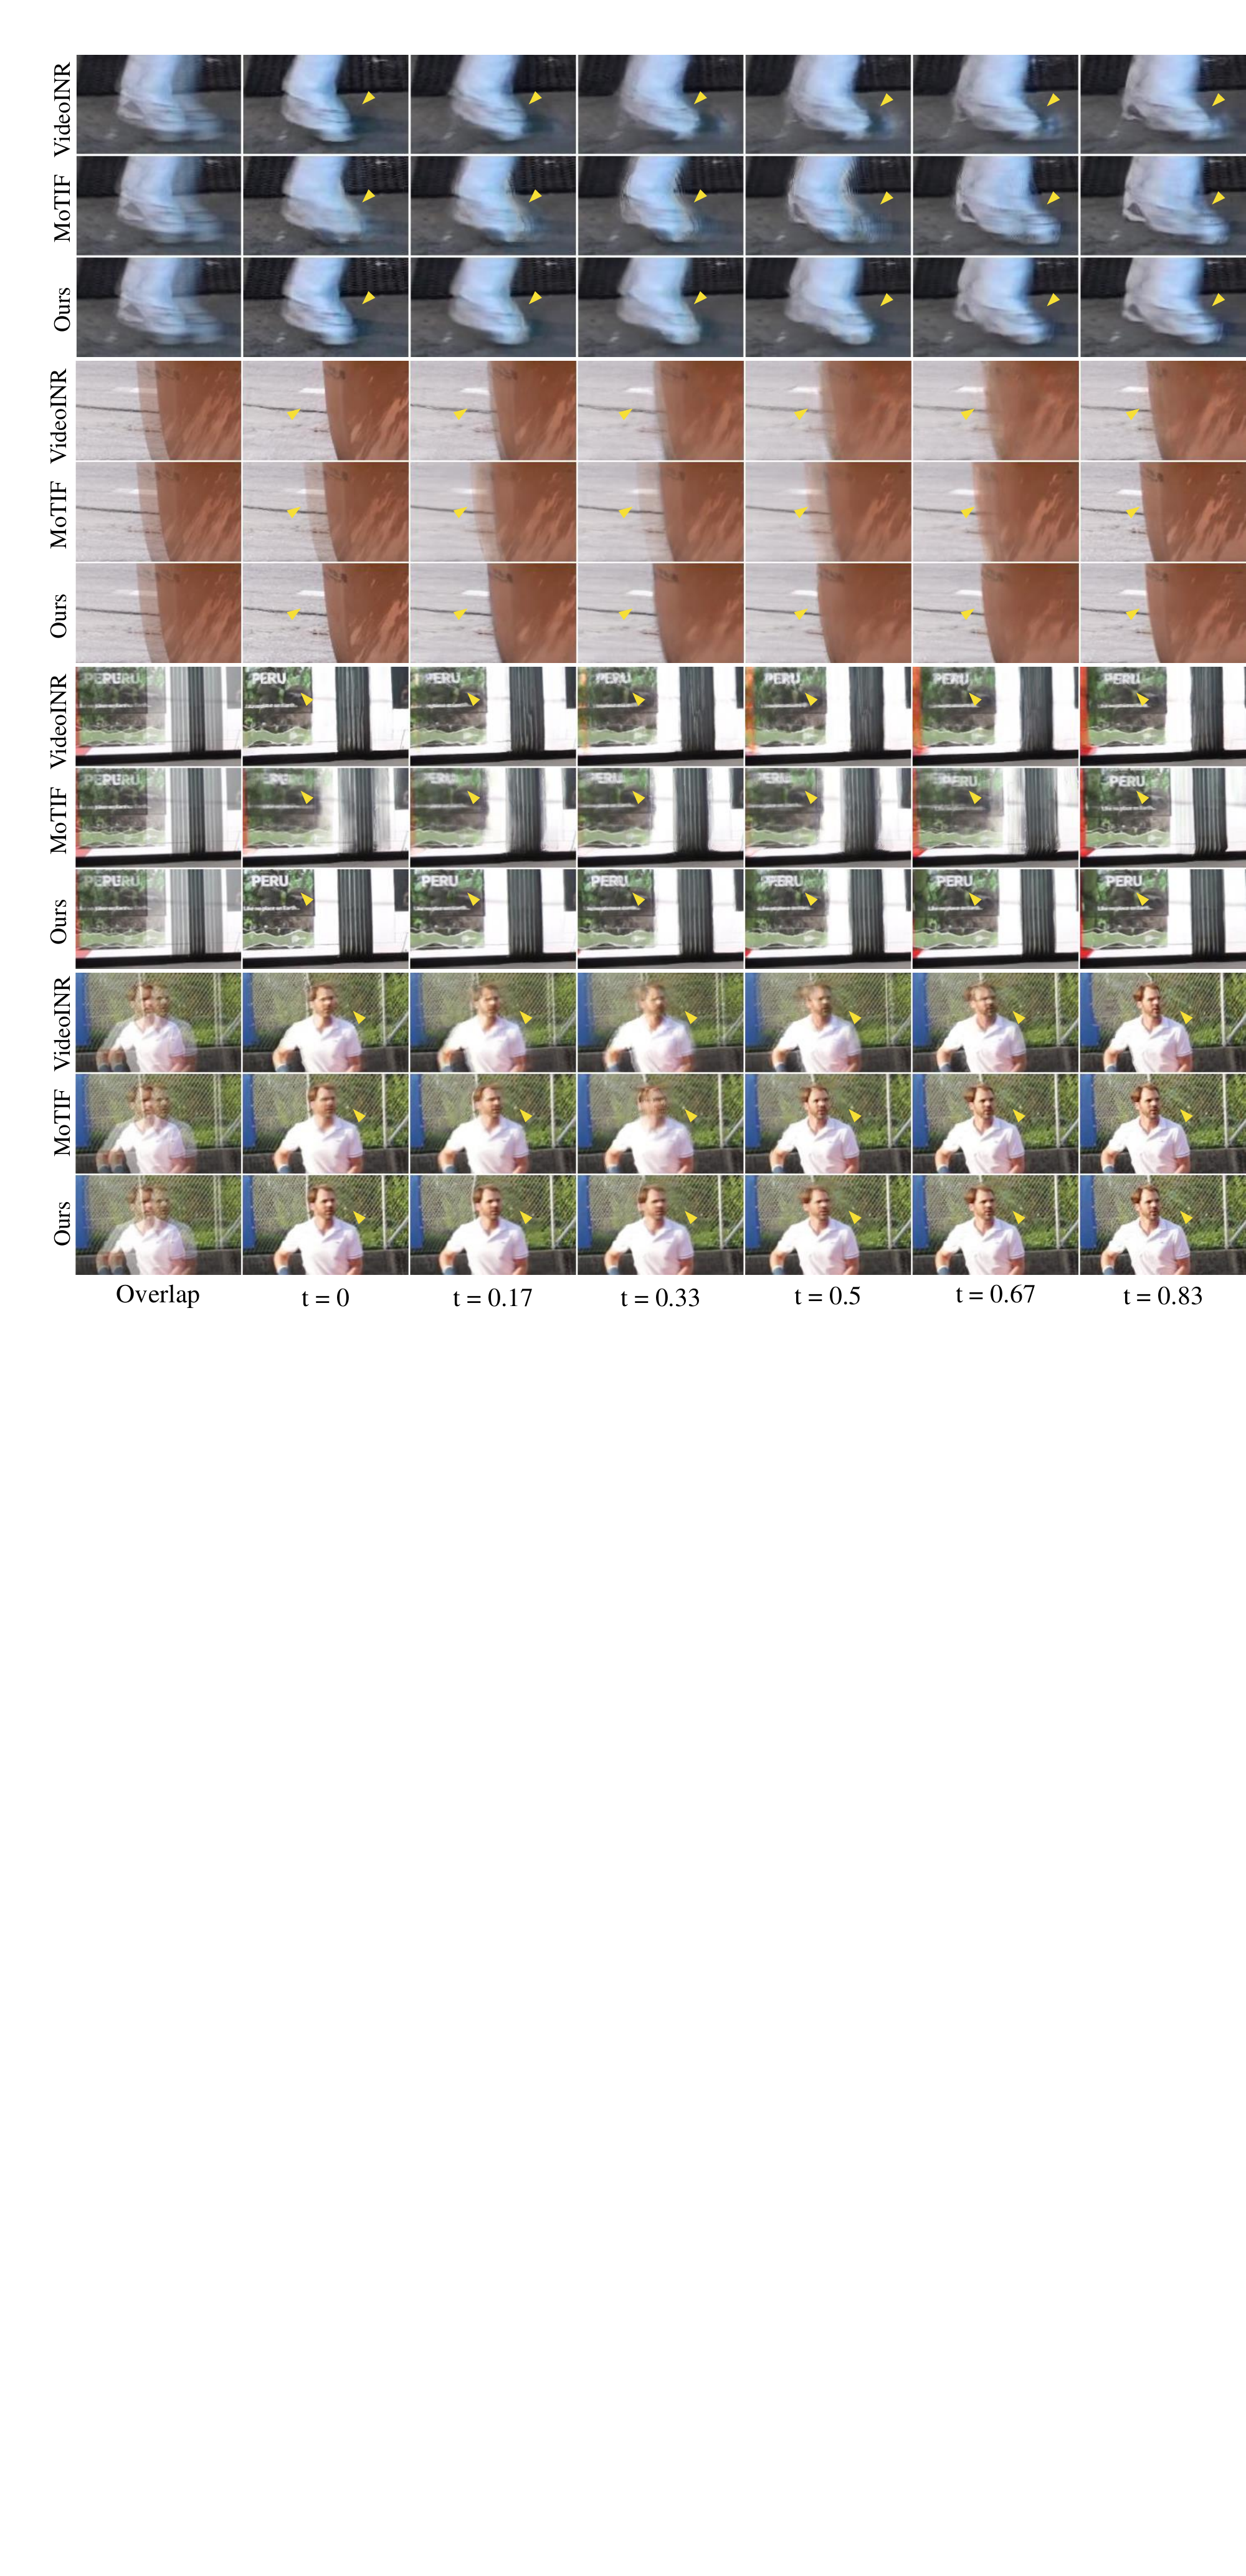}}
    \caption{Qualitative comparison on arbitrary scale temporal interpolation on out-of-distribution ($\times$6) with all time coordinates. We use the DAVIS dataset for evaluation. ``Overlap'' refers to the averaged image of two input frames ($t=0,1$), and the following images are interpolation results at $t=(0,1)$.  }
    
    \label{figure_x6} 
\end{figure*}
\clearpage

%-------------------------------------------------------------------------

\begin{figure*}[!t]
    \centerline{\includegraphics[width=\linewidth]{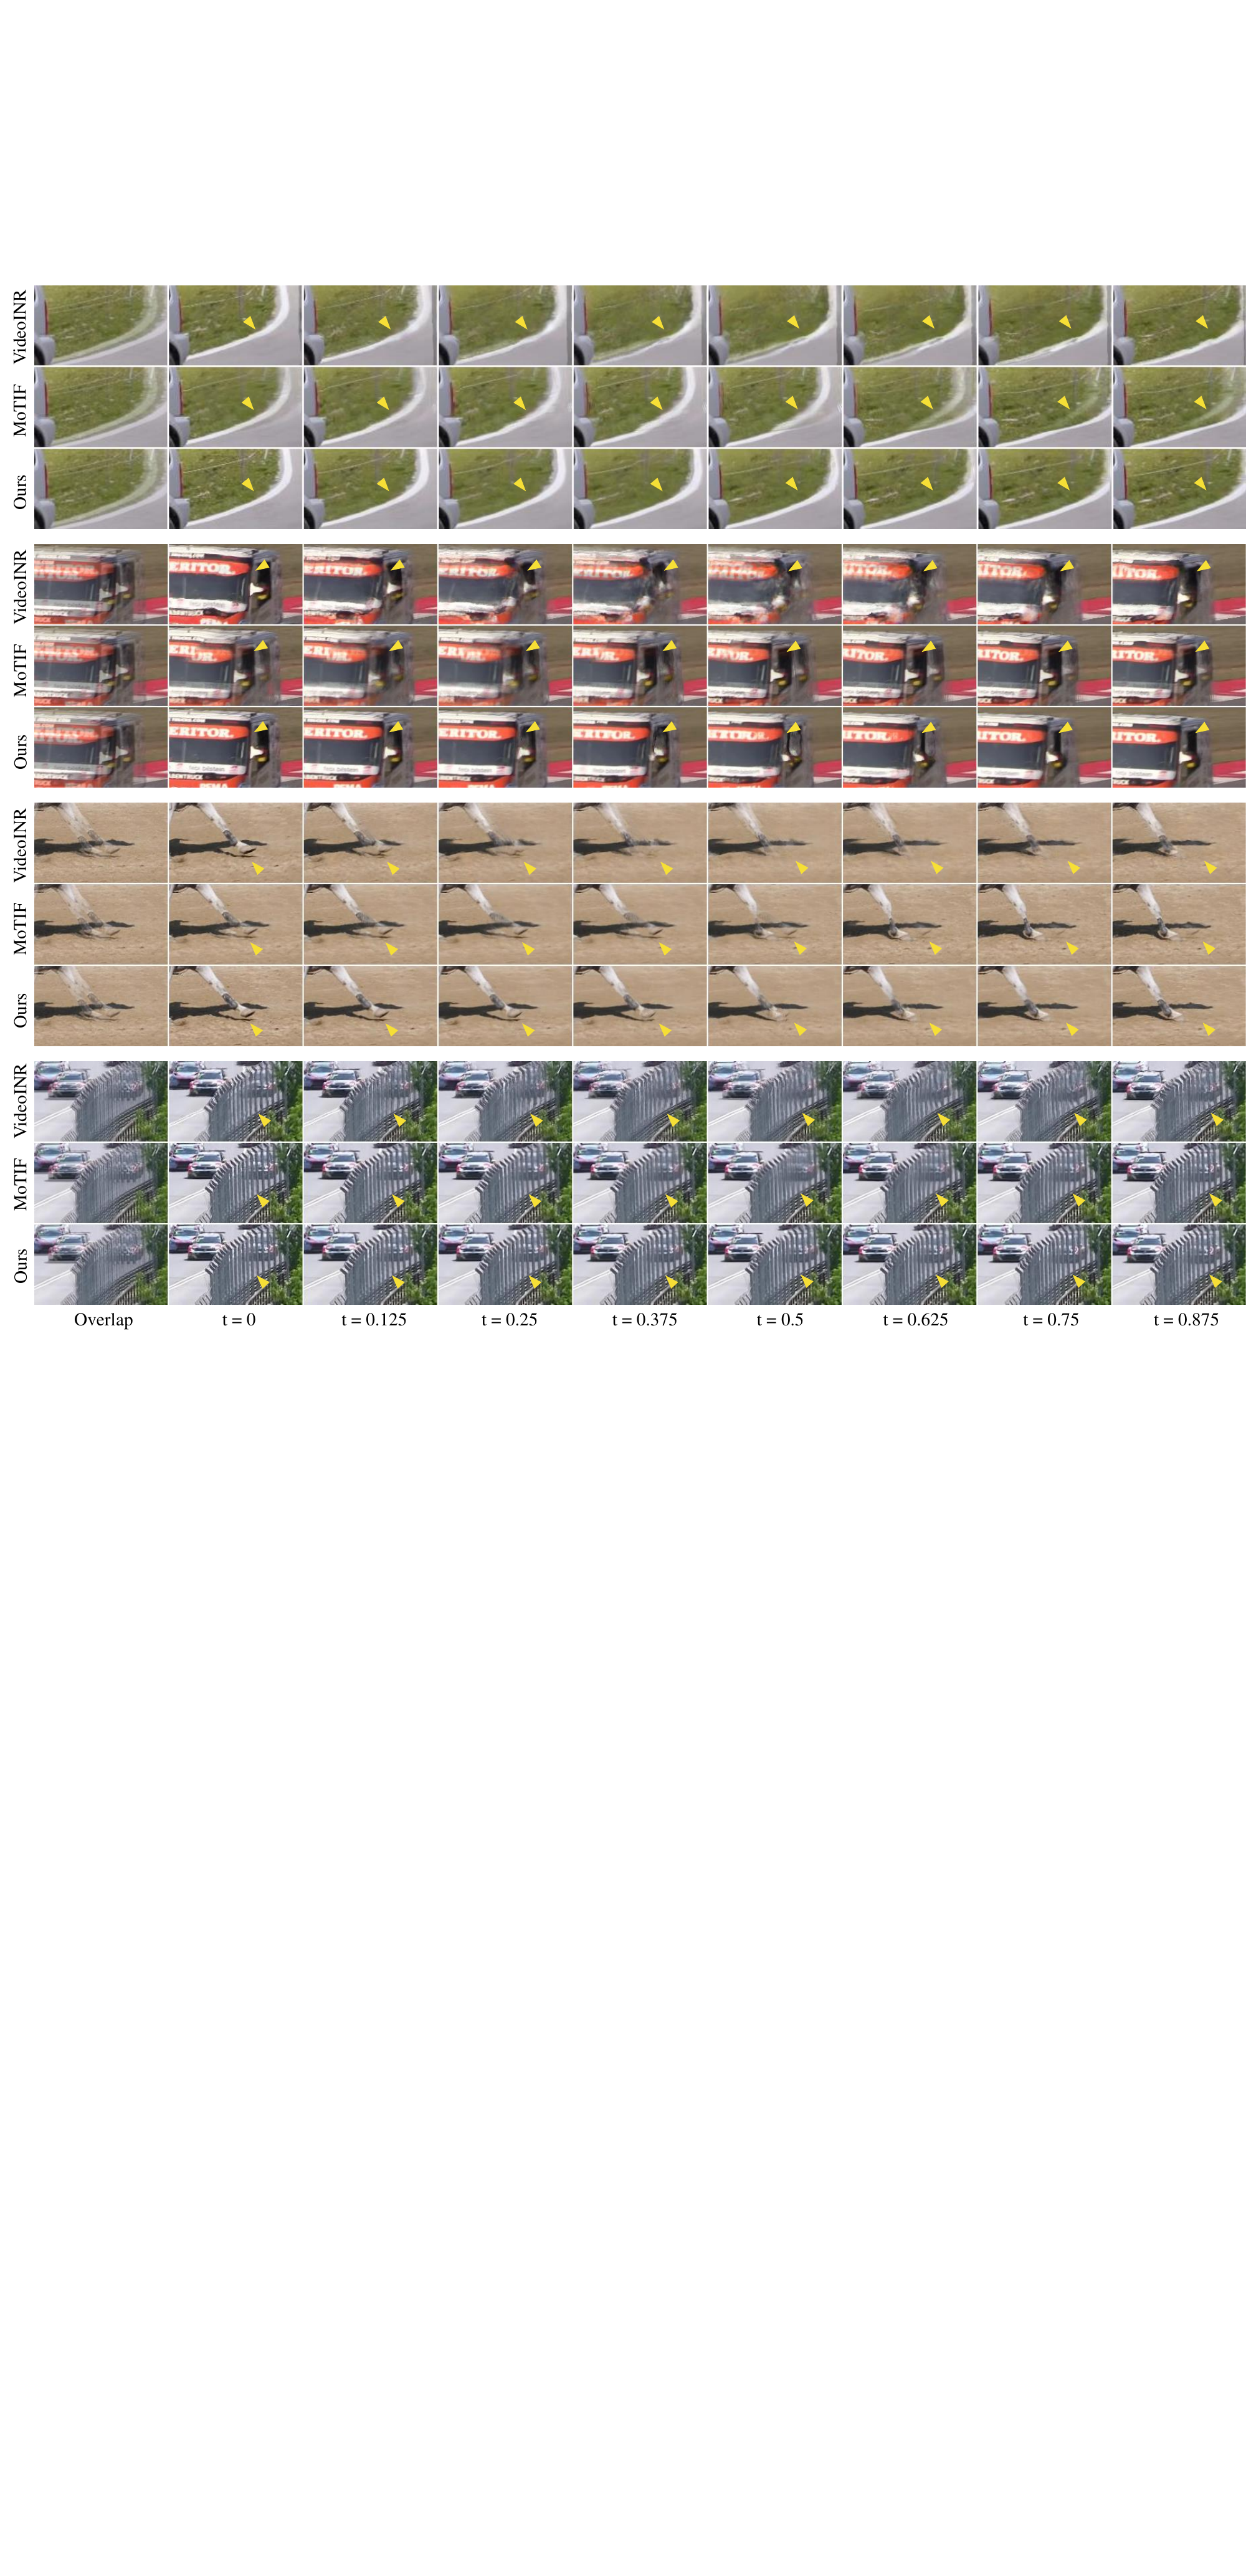}}
    \caption{Qualitative comparison on arbitrary scale temporal interpolation on in-distribution ($\times$8) with all time coordinates. We use the DAVIS dataset for evaluation. ``Overlap'' refers to the averaged image of two input frames ($t=0,1$), and the following images are interpolation results at $t=(0,1)$.  }
    
    \label{figure_x8} 
\end{figure*}
\clearpage
%-------------------------------------------------------------------------

\begin{figure*}[!t]
    \centerline{\includegraphics[width=\linewidth]{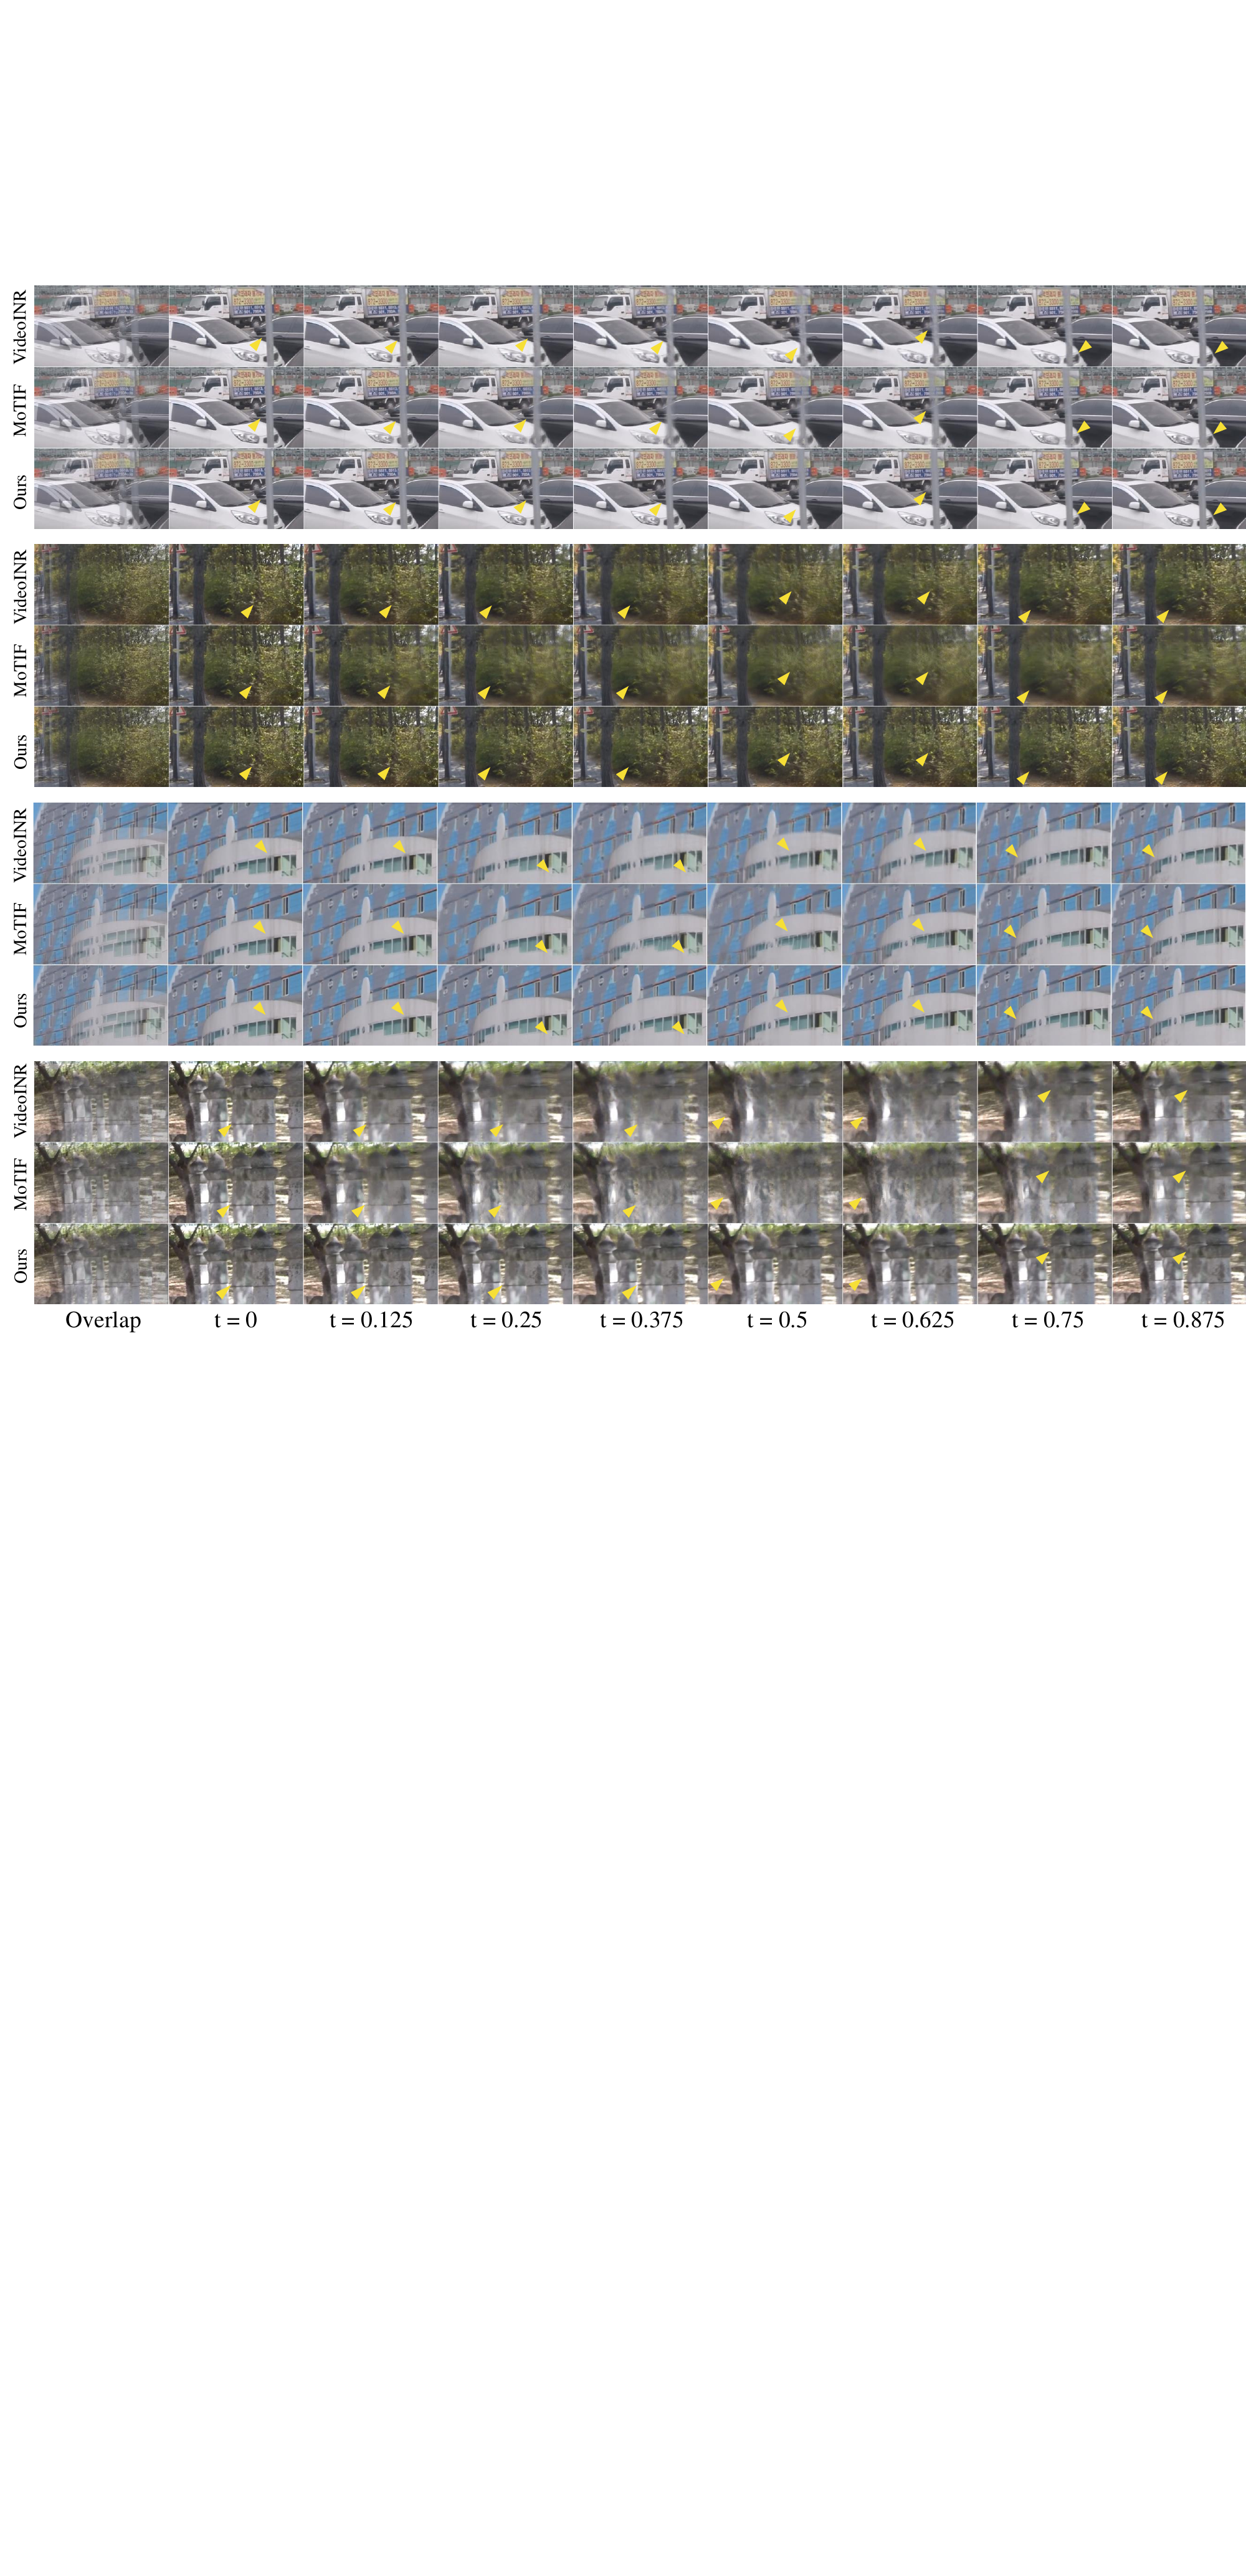}}
    \caption{Qualitative comparison on arbitrary scale temporal interpolation on in-distribution ($\times$8) for temporal scale and in-distribution ($\times$4) for spatial scale with all time coordinates. We use the DAVIS dataset for evaluation. ``Overlap'' refers to the averaged image of two input frames ($t=0,1$), and the following images are interpolation results at $t=(0,1)$.  }
    
    \label{figure_gopro_x4x8} 
\end{figure*}
\clearpage

%-------------------------------------------------------------------------

\begin{figure*}[!t]
    \centerline{\includegraphics[width=\linewidth]{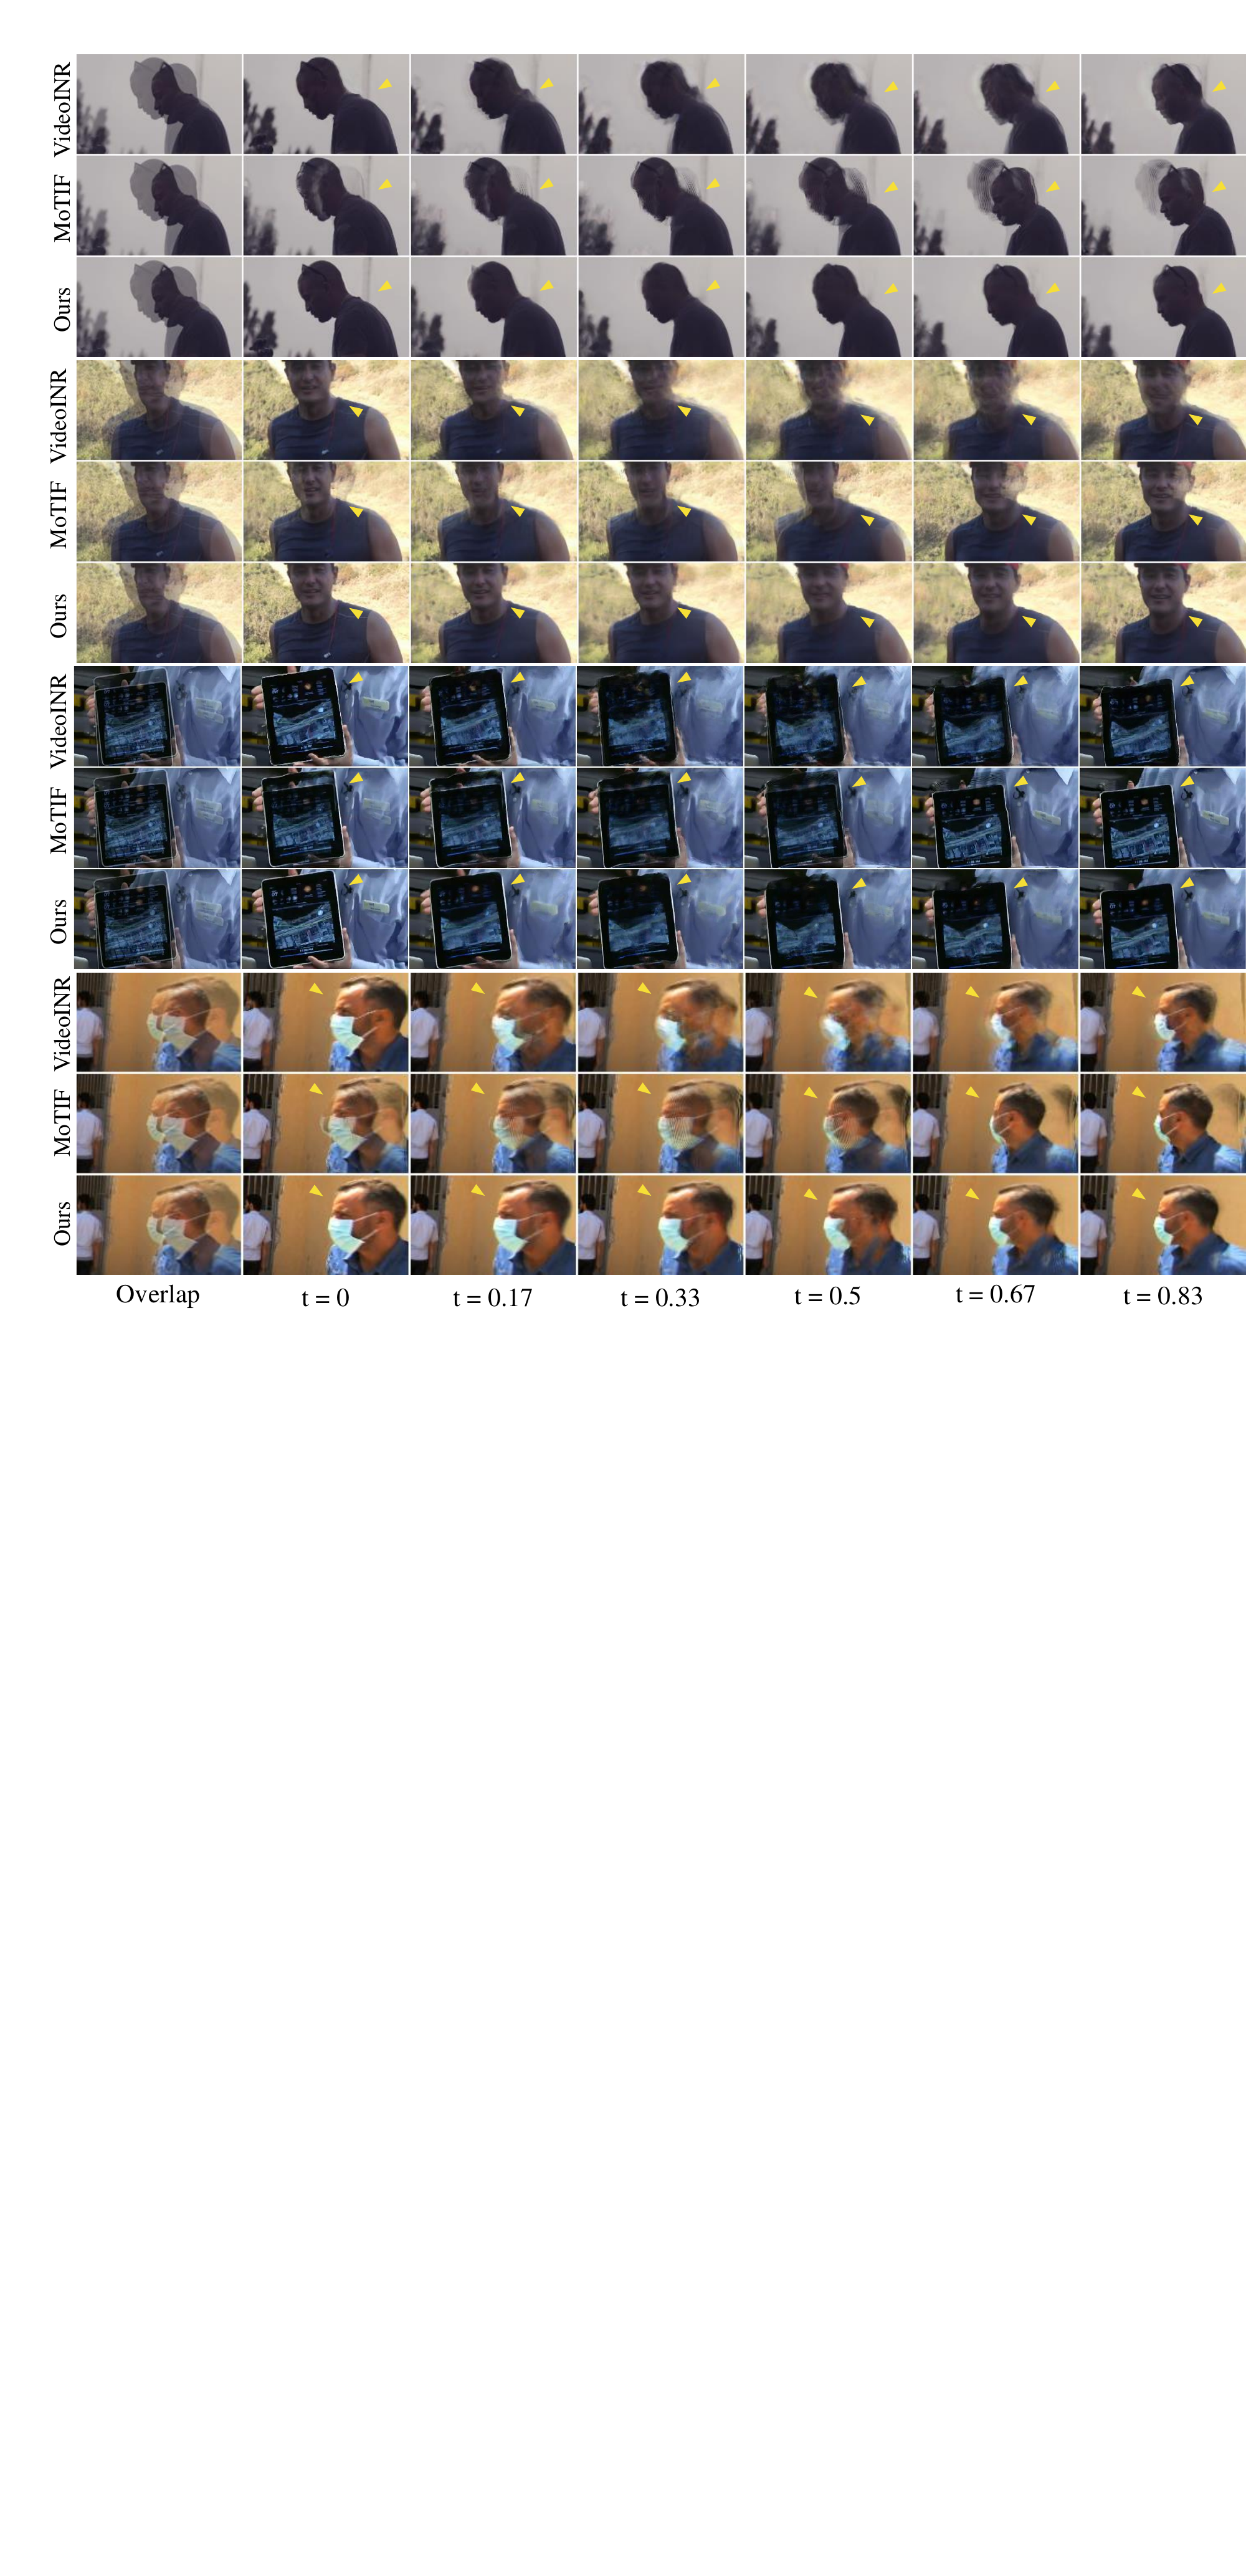}}
    \caption{Qualitative comparison on arbitrary scale temporal interpolation on out-of-distribution ($\times$6) with all time coordinates. We use the Vimeo-medium testset for evaluation. ``Overlap'' refers to the averaged image of two input frames ($t=0,1$), and the following images are interpolation results at $t=(0,1)$.}
    
    \label{figure_vimeo_medium_x1x6} 
\end{figure*}
\clearpage
%-------------------------------------------------------------------------

%-------------------------------------------------------------------------

\begin{figure*}[!t]
    \centerline{\includegraphics[width=\linewidth]{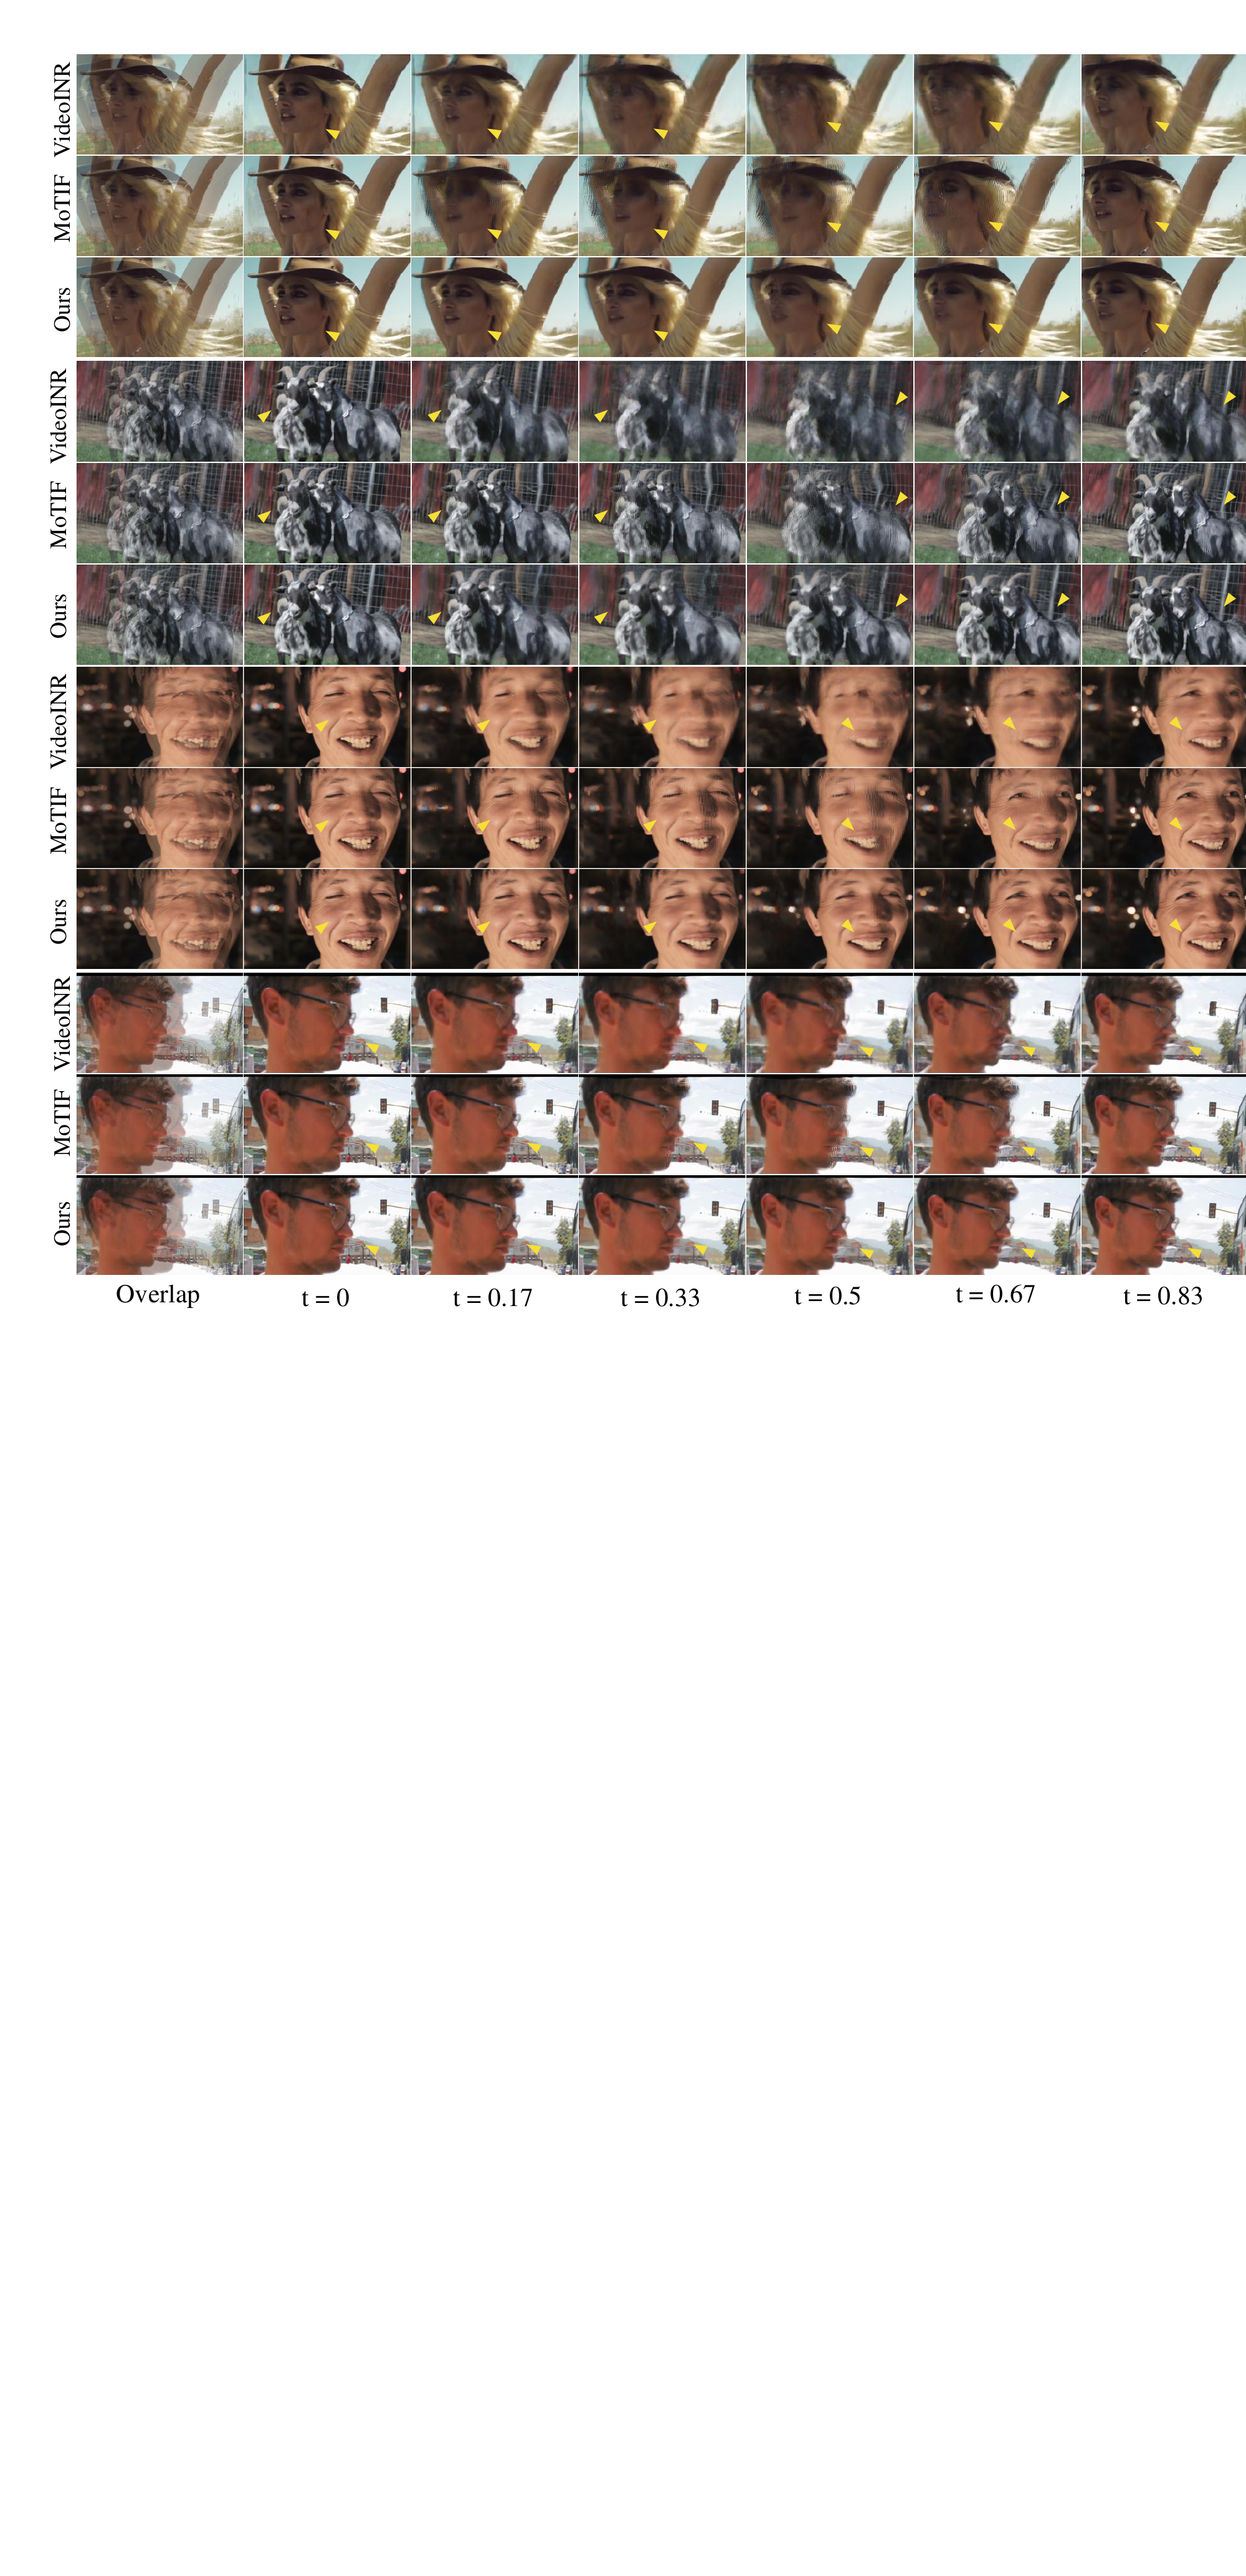}}
    \caption{Qualitative comparison on arbitrary scale spatio-temporal interpolation on out-of-distribution ($\times$6) for temporal scale and out-of-distribution ($\times$2) for spatial scale with all time coordinates. We use the Vimeo-Fast testset for evaluation. ``Overlap'' refers to the averaged image of two input frames ($t=0,1$), and the following images are interpolation results at $t=(0,1)$.}
    
    \label{figure_vimeo_fast_x2x6} 
\end{figure*}
\clearpage
%-------------------------------------------------------------------------

%-------------------------------------------------------------------------

\begin{figure*}[!t]
    \centerline{\includegraphics[width=\linewidth]{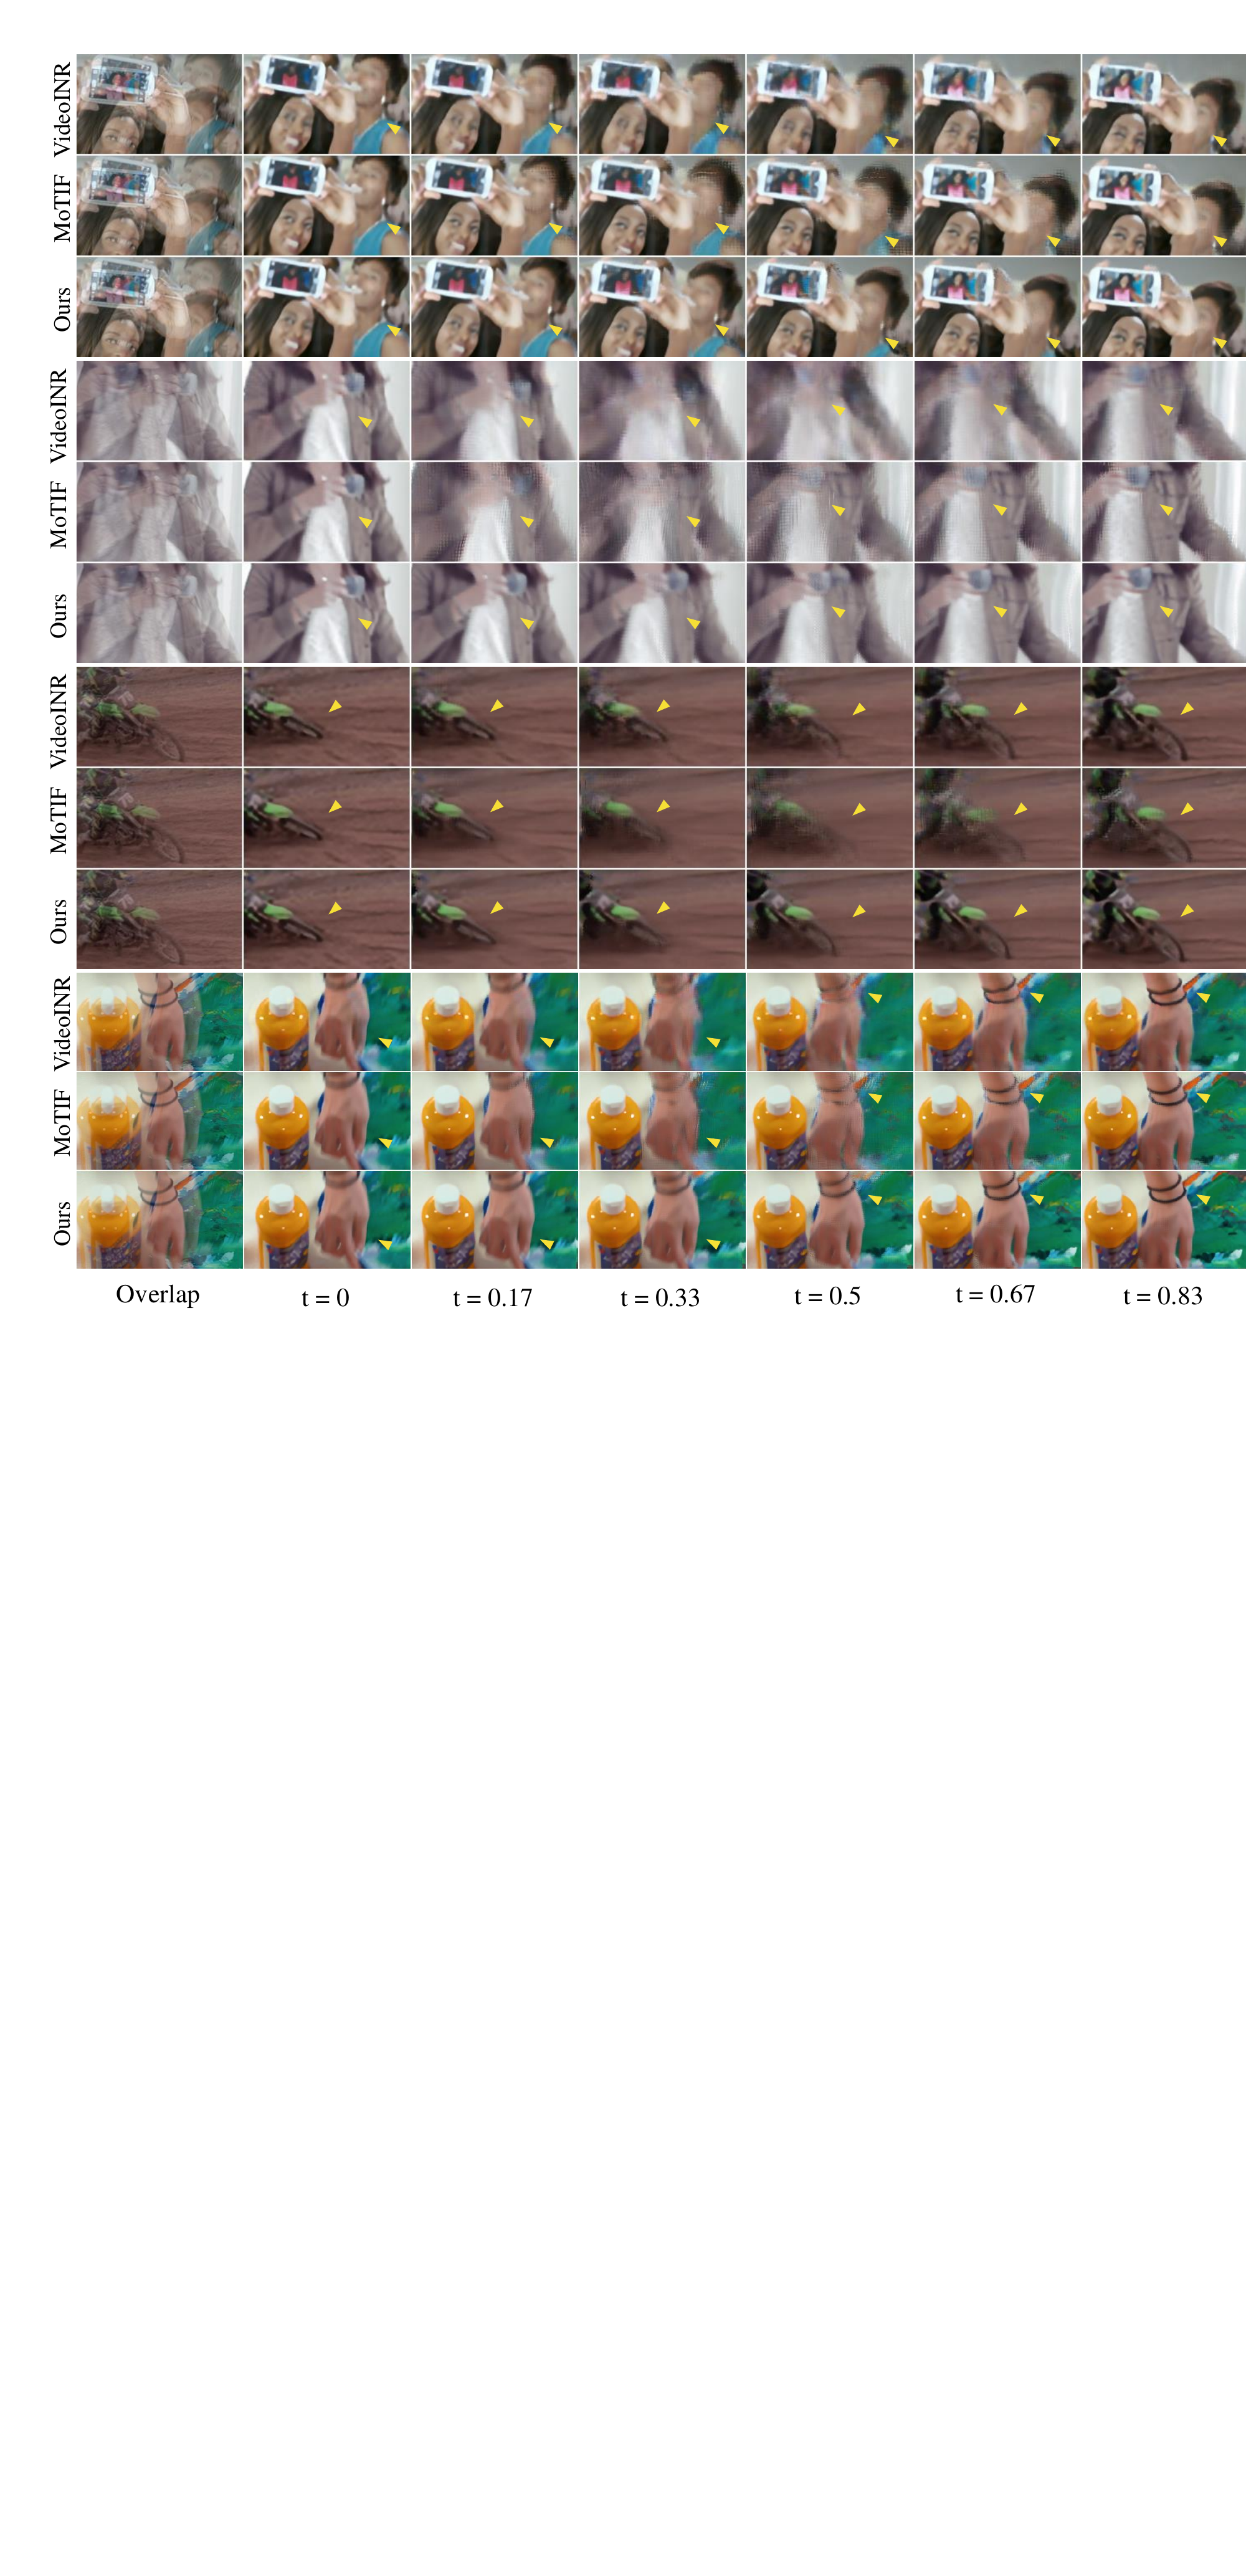}}
    \caption{Qualitative comparison on arbitrary scale spatio-temporal interpolation on out-of-distribution ($\times$6) for temporal scale and out-of-distribution ($\times$4) for spatial scale with all time coordinates. We use the Vimeo-Fast testset for evaluation. ``Overlap'' refers to the averaged image of two input frames ($t=0,1$), and the following images are interpolation results at $t=(0,1)$.}
    
    \label{figure_vimeo_fast_x4x6} 
\end{figure*}
\clearpage
%-------------------------------------------------------------------------
